# Supplementary material for: Correlated Quantal Response Equilibrium: A New Equilibrium Notion for Human-AI Strategic Interactions
Source: arXiv:2610.29020 source file (2026-10-21)
Supplement: Supplementary file 1 [file attempt2.tex]

\documentclass[11pt]{article}

\usepackage{amsmath,amssymb,amsthm}
\usepackage{geometry}
\geometry{margin=1in}

\begin{document}

\paragraph{Attempt 2}
Let
\[
\rho \in \Delta(\mathcal A_1 \times \mathcal A_2)
\]
be a candidate joint distribution over action pairs.

For each player, define the set of deviation maps
\begin{align}
\Phi_1 &:= \{\phi_1 : \mathcal A_1 \to \mathcal A_1\},
\label{eq:phi_space_1}
\\
\Phi_2 &:= \{\phi_2 : \mathcal A_2 \to \mathcal A_2\}.
\label{eq:phi_space_2}
\end{align}

Let $\mathrm{id}_1 \in \Phi_1$ and $\mathrm{id}_2 \in \Phi_2$ denote the identity maps,
\[
\mathrm{id}_1(a_1)=a_1,
\qquad
\mathrm{id}_2(a_2)=a_2,
\]


For Player~1, define the value of a deviation map $\phi_1$ under $\rho$ by
\begin{align}
U_1(\phi_1;\rho)
&:=
\sum_{a_1 \in \mathcal A_1}\sum_{a_2 \in \mathcal A_2}
\rho(a_1,a_2)\,R_1(\phi_1(a_1),a_2).
\label{eq:map_value_1}
\end{align}

Similarly, for Player~2,
\begin{align}
U_2(\phi_2;\rho)
&:=
\sum_{a_1 \in \mathcal A_1}\sum_{a_2 \in \mathcal A_2}
\rho(a_1,a_2)\,R_2(a_1,\phi_2(a_2)).
\label{eq:map_value_2}
\end{align}

Define the deviation gains relative to obedience, which is the gap between what one change action and one does not change action:
\begin{align}
\Delta_1(\phi_1;\rho)
&:=
U_1(\phi_1;\rho)-U_1(\mathrm{id}_1;\rho),
\label{eq:map_gain_1}
\\
\Delta_2(\phi_2;\rho)
&:=
U_2(\phi_2;\rho)-U_2(\mathrm{id}_2;\rho).
\label{eq:map_gain_2}
\end{align}

\paragraph{Correlated equilibrium in deviation-map form}

Since
\[
U_1(\mathrm{id}_1;\rho)
=
\sum_{a_1,a_2}\rho(a_1,a_2)R_1(a_1,a_2),
\qquad
U_2(\mathrm{id}_2;\rho)
=
\sum_{a_1,a_2}\rho(a_1,a_2)R_2(a_1,a_2),
\]
the correlated-equilibrium constraints can be written as
\begin{align}
U_1(\mathrm{id}_1;\rho)
&\ge
U_1(\phi_1;\rho),
\qquad
\forall \phi_1 \in \Phi_1,
\label{eq:ce_map_p1}
\\
U_2(\mathrm{id}_2;\rho)
&\ge
U_2(\phi_2;\rho),
\qquad
\forall \phi_2 \in \Phi_2.
\label{eq:ce_map_p2}
\end{align}

Equivalently,
\begin{align}
\Delta_1(\phi_1;\rho) &\le 0,
\qquad \forall \phi_1 \in \Phi_1,
\label{eq:ce_map_gain_p1}
\\
\Delta_2(\phi_2;\rho) &\le 0,
\qquad \forall \phi_2 \in \Phi_2.
\label{eq:ce_map_gain_p2}
\end{align}

\paragraph{Quantal response over deviation maps}

Fix an temperature parameter $\theta > 0$.
We define the quantal response of Player~1 over the deviation-map space $\Phi_1$ by
\begin{align}
\Lambda_1^\theta(\phi_1 \mid \rho)
&:=
\frac{\exp\!\big(\theta\,\Delta_1(\phi_1;\rho)\big)}
{\sum_{\psi_1 \in \Phi_1}\exp\!\big(\theta\,\Delta_1(\psi_1;\rho)\big)},
\qquad \phi_1 \in \Phi_1.
\label{eq:qr_map_1}
\end{align}

Similarly, for Player~2,
\begin{align}
\Lambda_2^\theta(\phi_2 \mid \rho)
&:=
\frac{\exp\!\big(\theta\,\Delta_2(\phi_2;\rho)\big)}
{\sum_{\psi_2 \in \Phi_2}\exp\!\big(\theta\,\Delta_2(\psi_2;\rho)\big)},
\qquad \phi_2 \in \Phi_2.
\label{eq:qr_map_2}
\end{align}

We can then get the induced action-level response, and the joint distribution.


\paragraph{Induced action-level response kernels}

For Player~1,
let
\begin{align}
Q_1^\theta(a_1' \mid a_1;\rho)
&:=
\sum_{\phi_1 \in \Phi_1}
\Lambda_1^\theta(\phi_1 \mid \rho)\,
\mathbf{1}\{\phi_1(a_1)=a_1'\},
\label{eq:action_kernel_1}
\end{align}
and similarly, for Player~2,
\begin{align}
Q_2^\theta(a_2' \mid a_2;\rho)
&:=
\sum_{\phi_2 \in \Phi_2}
\Lambda_2^\theta(\phi_2 \mid \rho)\,
\mathbf{1}\{\phi_2(a_2)=a_2'\}.
\label{eq:action_kernel_2}
\end{align}

$Q_1^\theta(a_1' \mid a_1;\rho)$ is the probability that Player 1
actually plays $a_1'$ when intially want to play $a_1$.

\paragraph{Induced joint and correlated quantal response equilibrium}

Starting from $\rho$, first draw $(a_1,a_2) \sim \rho$, then let each player
transform the recommended (initial) action according to the induced 
$Q_1^\theta(\cdot \mid a_1;\rho)$ and $Q_2^\theta(\cdot \mid a_2;\rho)$.
This yields a new joint distribution $T_\theta(\rho)$ on
$\mathcal A_1 \times \mathcal A_2$:
\begin{align}
(T_\theta \rho)(a_1',a_2')
&:=
\sum_{a_1 \in \mathcal A_1}\sum_{a_2 \in \mathcal A_2}
\rho(a_1,a_2)\,
Q_1^\theta(a_1' \mid a_1;\rho)\,
Q_2^\theta(a_2' \mid a_2;\rho).
\label{eq:T_theta_def}
\end{align}

We say that
\[
\rho^\theta \in \Delta(\mathcal A_1 \times \mathcal A_2)
\]
is a correlated quantal response equilibrium if it is a fixed point of
$T_\theta$, i.e.,
\begin{align}
\rho^\theta
&=
T_\theta(\rho^\theta).
\label{eq:cqre_fixed_point}
\end{align}




\end{document}
