# Supplementary material for: Correlated Quantal Response Equilibrium: A New Equilibrium Notion for Human-AI Strategic Interactions
Source: arXiv:2610.29020 source file (2026-10-21)
Supplement: Supplementary file 2 [file drafts.tex]

\documentclass[11pt]{article}

% --- Core math & symbols --- 
\usepackage{amsmath, amssymb, amsfonts, mathtools}
\usepackage{bm}
\usepackage{amsthm}
\newtheorem{proposition}{Proposition}

% ---- theorem environments (add in preamble) ----
\usepackage{amsthm}   % provides \newtheorem and the definition environment
\usepackage{amsmath}  % provides align/equation environments
\usepackage{amssymb}  % provides \Delta and other symbols
\newtheorem{theorem}{Theorem}

\newtheorem{definition}{Definition}
%\newtheorem{proposition}{Proposition}


% --- Tables & figures ---
\usepackage{graphicx}
\usepackage{booktabs}
\usepackage{array}
\usepackage{caption}
\captionsetup{font=small}

% --- Typography & layout ---
\usepackage[margin=1in]{geometry}
\usepackage{microtype}
\usepackage{lmodern}
\usepackage{xcolor}

% --- Hyperlinks & clever references ---
\usepackage[hidelinks]{hyperref}
\usepackage[nameinlink]{cleveref}

% --- Handy macros ---
\newcommand{\Unif}{\mathrm{Unif}}
\newcommand{\QBR}{\mathrm{QBR}}
\newcommand{\E}{\mathbb{E}}
\newcommand{\R}{\mathbb{R}}
\newcommand{\Aone}{\mathcal{A}_1}
\newcommand{\Atwo}{\mathcal{A}_2}

\usepackage{color-edits}
\addauthor[VS]{vs}{magenta}
\addauthor[AZ]{az}{blue}

\title{\texttt{learn\_eq}}
\author{Andy}
\date{October 2025}

\begin{document}
\maketitle

\section{Method}

We consider a two-player normal-form game with finite action sets 
\(A_1=\{1,\dots,K_1\}\) and \(A_2=\{1,\dots,K_2\}\),
and payoff matrices \(u_1, u_2\).


\subsection{Data Generation}
We generate trajectories using \textit{fictitious play} dynamics.
At each iteration \(t\), players update beliefs over opponent actions and respond
with soft best responses:
\begin{equation}
\begin{aligned}
a_2' &\sim FP_2^{(t-1)}, &
a_1 &\sim \mathrm{Softmax}_{a_1}\!\big(u_1(a_1,a_2') / \tau_1 \big),\\
a_1' &\sim FP_1^{(t-1)}, &
a_2 &\sim \mathrm{Softmax}_{a_2}\!\big(u_2(a_1',a_2) / \tau_2 \big),
\end{aligned}
\end{equation}
belief updates:
\begin{equation}
FP_i^{(t)} = \alpha FP_i^{(t-1)} + (1-\alpha)\,\delta_{a_i}.
\end{equation}
The resulting dataset 
\(D = \{(a_1^{(i)}, a_2^{(i)})\}_{i=1}^N\)


\subsection{Neural Behavior Models (Player-1 Perspective)}
Player~1 maintains two neural components:

\paragraph{Opponent model (\( \mathrm{NN}_{2'} \)).}
An unconditional belief distribution over opponent actions:
\begin{equation}
p_{\theta_{2'}}(a_2)
= \mathrm{Softmax}(z_{\theta_{2'}}),
\end{equation}
where \(z_{\theta_{2'}} \in \mathbb{R}^{K_2}\) are learnable logits.
The model is trained by maximum likelihood:
\begin{equation}
\mathcal{L}_{2'}(\theta_{2'})
= -\frac{1}{N}\sum_{i=1}^N \log p_{\theta_{2'}}(a_2^{(i)}).
\end{equation}

\paragraph{Best-response model (\( \mathrm{NN}_1 \)).}
A conditional policy mapping opponent actions to self-actions:
\begin{equation}
p_{\theta_1}(a_1 \mid a_2)
= \mathrm{Softmax}\!\big(f_{\theta_1}(a_2)\big),
\end{equation}
optimized under the objective:
\begin{equation}
\mathcal{L}_1(\theta_1)
= -\frac{1}{N}\sum_{i=1}^N \log p_{\theta_1}(a_1^{(i)} \mid a_2^{(i)}).
\end{equation}

\subsection{Inference Procedure}
At decision time, Player~1 performs a single reasoning step:
\begin{equation}
\begin{aligned}
a_1' &\sim \mathrm{Unif}(A_1),\\
u &\sim \mathrm{Unif}(0,1), \quad
a_2' = F_{p_{\theta_{2'}}}^{-1}(u),\\
a_1 &\sim p_{\theta_1}(\cdot \mid a_2'),
\end{aligned}
\end{equation}
where \(F_{p_{\theta_{2'}}}^{-1}\) denotes inverse-CDF sampling from the learned belief.
The resulting triple \((a_1', a_2', a_1)\) expresses the reasoning chain:
\emph{``if I were to play \(a_1'\), I believe the opponent would play \(a_2'\); 
therefore I act as \(a_1\).''}



\pagebreak

\section{New Methods}
\subsection{Neural Behavior Model (Revised, Player-1 Perspective)}
Player~1 maintains a single neural model representing the opponent's conditional behavior and computes its own best response analytically from the game payoff.

\paragraph{Conditional opponent model (\( \mathrm{NN}_{2'} \)).}
Rather than modeling an unconditional belief over \(a_2\),
Player~1 learns a conditional distribution
capturing how the opponent reacts to each possible self-action:
\begin{equation}
p_{\theta_{2'}}(a_2 \mid a_1)
= \mathrm{Softmax}\!\big(f_{\theta_{2'}}(a_1)\big),
\end{equation}
where \(f_{\theta_{2'}}: \mathcal{A}_1 \to \mathbb{R}^{K_2}\) 
is a neural network producing logits over opponent actions.
The network is trained from observed play data 
\(\mathcal{D}=\{(a_1^{(i)},a_2^{(i)})\}_{i=1}^N\)
by maximum likelihood:
\begin{equation}
\mathcal{L}_{2'}(\theta_{2'})
= -\frac{1}{N}\sum_{i=1}^N 
\log p_{\theta_{2'}}(a_2^{(i)} \mid a_1^{(i)}).
\end{equation}
This model approximates the opponent’s empirical best-response distribution.

\paragraph{Analytical best response (replace \( \mathrm{NN}_1 \)).}
Given the learned belief \(p_{\theta_{2'}}(a_2 \mid a_1)\)
and Player~1’s known utility function \(U_1(a_1,a_2)\),
the expected utility for each action is computed as
\begin{equation}
J_1(a_1)
= \mathbb{E}_{a_2 \sim p_{\theta_{2'}}(\cdot \mid a_1)}
  [\,U_1(a_1,a_2)\,]
= \sum_{a_2 \in \mathcal{A}_2}
  p_{\theta_{2'}}(a_2 \mid a_1)\, U_1(a_1,a_2).
\end{equation}
The best-response policy of Player~1 is then defined by either
\begin{equation}
a_1^* = \arg\max_{a_1 \in \mathcal{A}_1} J_1(a_1),
\end{equation}
or, under a logit (soft) model of bounded rationality,
\begin{equation}
p^*(a_1) 
\propto \exp\!\big(\beta_1 J_1(a_1)\big),
\end{equation}
where \(\beta_1>0\) controls the degree of stochasticity.

\subsection{Inference Procedure}
At decision time, Player~1 evaluates all candidate actions 
through its learned opponent model and payoff matrix:
\begin{equation}
\begin{aligned}
a_2' &\sim p_{\theta_{2'}}(\cdot \mid a_1),
\quad J_1(a_1) = \sum_{a_2} p_{\theta_{2'}}(a_2 \mid a_1) U_1(a_1,a_2),\\
a_1^* &= \arg\max_{a_1} J_1(a_1),
\end{aligned}
\end{equation}
which corresponds to the reasoning statement:
\emph{``If I were to play \(a_1\), I believe the opponent would respond as \(p_{\theta_{2'}}(a_2 \mid a_1)\);
therefore I act as \(a_1^*\) that maximizes my expected utility.''}

\paragraph{change}
Compared to the previous framework, 
the unconditional belief \(p_{\theta_{2'}}(a_2)\) is replaced by the 
conditional response model \(p_{\theta_{2'}}(a_2 \mid a_1)\),
and the neural best-response model \(p_{\theta_1}(a_1 \mid a_2)\)
is replaced by an explicit optimization over the known utility \(U_1(a_1,a_2)\).
The data generation process (\emph{e.g.}, stochastic fictitious play)
remains unchanged.

\pagebreak









\section{Offline Behavioral Data Generation Design}

We consider a two–player setting with action sets
\[
\mathcal A_1=\{A,B\}, \qquad
\mathcal A_2=\{L,R\}.
\]
Player~1 (P1) samples actions from a mixed strategy
$\pi_1\in\Delta(\mathcal A_1)$,
while Player~2 (P2) responds according to a behavioral kernel
$W\in\mathbb R^{|\mathcal A_1|\times|\mathcal A_2|}$ and rationality parameter
$\lambda>0$.
For any belief $\pi_1'$, P2’s quantal–response policy is
\[
\pi_2(\cdot\mid\pi_1',\lambda)
=\operatorname{softmax}\!\big(\lambda\, W^\top \pi_1'\big),
\qquad
\pi_2(j\mid\pi_1',\lambda)
=\frac{\exp\{\lambda (W^\top\pi_1')_j\}}
      {\sum_k\exp\{\lambda (W^\top\pi_1')_k\}}.
\]
We generate offline behavioral data by specifying how $\pi_1'$ (the belief
used by P2) relates to the true $\pi_1$ used by P1.  Three natural variants
are described below.

\subsection{Variant I: Independent Beliefs}
At each round:
\begin{enumerate}
\item Sample P1's policy $\pi_1\sim\operatorname{Dirichlet}(\alpha)$.
\item Draw $A_1\sim\pi_1$.
\item Independently draw P2's belief $\pi_1'\sim\operatorname{Dirichlet}(\alpha')$.
\item Compute $\pi_2=\operatorname{softmax}(\lambda W^\top\pi_1')$
      and sample $A_2\sim\pi_2$.
\end{enumerate}


\subsection{Variant II: Shared Prior ($\pi_1'=\pi_1$)}
Here P2's belief equals P1's actual mixed strategy.
For each context $c$:
\begin{enumerate}
\item Sample a fixed $\pi_1^{(c)}\!\sim\!\operatorname{Dirichlet}(\alpha)$
      and hold it for $T_c$ rounds.
\item For each round $t$:
      draw $A_{1,t}\!\sim\!\pi_1^{(c)}$,
      set $\pi_2^{(c)}=\operatorname{softmax}(\lambda W^\top\pi_1^{(c)})$,
      and draw $A_{2,t}\!\sim\!\pi_2^{(c)}$.
\end{enumerate}


\subsection{Variant III: Anchored Noisy Beliefs}
To capture partially correct beliefs, we let P2’s belief be a noisy version
of $\pi_1$:
\[
\pi_1'\sim\operatorname{Dirichlet}(\kappa\,\pi_1),
\]
where $\kappa>0$ controls P2’s confidence.
As $\kappa\!\to\!\infty$, $\pi_1'\!\approx\!\pi_1$ (well-informed P2);
for small $\kappa$, $\pi_1'$ becomes diffuse (misinformed P2).
The generation steps are:
\begin{enumerate}
\item Sample $\pi_1\sim\operatorname{Dirichlet}(\alpha)$ and
      $A_1\sim\pi_1$.
\item Sample $\pi_1'\sim\operatorname{Dirichlet}(\kappa\pi_1)$.
\item Compute $\pi_2=\operatorname{softmax}(\lambda W^\top\pi_1')$
      and draw $A_2\sim\pi_2$.
\end{enumerate}

\subsection{Observed--Action Design.}
In this variant, Player~2 no longer responds to an inferred or sampled belief
$\pi_1'$ but instead conditions directly on the realized action $A_1$ taken by
Player~1 in each round.  Specifically, after drawing $A_1=i$,
Player~2 forms the quantal--response policy
\[
\pi_2(\cdot\mid A_1=i,\lambda)
=\operatorname{softmax}\!\big(\lambda\,W[i,:]\big),
\]
and then samples $A_2\!\sim\!\pi_2(\cdot\mid A_1=i,\lambda)$.
This design ensures that $A_2$ is statistically dependent on the observed
$A_1$, allowing the offline dataset to contain direct state--action pairs
$(A_1,A_2)$ that reveal the underlying behavioral kernel.
Consequently, a neural network trained on this data can accurately learn
the mapping $A_1\!\mapsto\!\pi_2(\cdot\mid A_1)$, unlike the previous
variants where $A_2$ depended only on block--level latent variables.

\subsection{Variant 5: Game-Aware Shared Prior with Noisy Kernel.}
We tie the behavioral kernel to the game by setting $W=\widetilde R_2$, where
$\widetilde R_2 = R_2 + \varepsilon$ and $\varepsilon_{ij}\sim\mathcal N(0,\sigma^2)$
is drawn once and held fixed throughout the experiment (modeling stable but
misspecified cognition). As in the shared-prior design, each context $c$
samples $\pi_1^{(c)}\!\sim\!\mathrm{Dirichlet}(\alpha)$ and holds it for $T_c$
rounds, while P2’s belief equals the truth ($\pi_1'=\pi_1^{(c)}$). P2 then
plays the quantal response
$\pi_2^{(c)}=\mathrm{softmax}\!\big(\lambda\,\widetilde R_2^{\!\top}\pi_1^{(c)}\big)$,
and actions are generated by $A_{1,t}\!\sim\!\pi_1^{(c)}$ and
$A_{2,t}\!\sim\!\pi_2^{(c)}$. Because $\pi_2^{(c)}$ is constant within a block
and depends on the (latent) mixture $\pi_1^{(c)}$, the offline dataset
$\{(A_{1,t},A_{2,t})\}$ contains limited conditional signal unless block
identity or recent $A_1$ frequencies are provided to the learner.

\subsection{Variant 6: Game-Aware Observed-Action with Noisy Kernel.}
Here we again set $W=\widetilde R_2=R_2+\varepsilon$ (same noise model as
above), but P2 conditions on the \emph{realized} action $A_1$ each round:
after observing $A_1=i$, P2 plays
$\pi_2(\cdot\mid A_1=i)=\mathrm{softmax}\!\big(\lambda\,\widetilde R_2[i,:]\big)$
and then $A_2\!\sim\!\pi_2(\cdot\mid A_1=i)$. P1’s actions $A_1$ may be drawn
i.i.d.\ from a base prior or via Dirichlet blocks; in either case, the mapping
$A_1\mapsto A_2$ is now directly encoded in the data, so a classifier trained
only on action pairs can consistently recover $p(A_2\!\mid\!A_1)$ up to the
softmax temperature and the misspecification level $\sigma$. This variant is
both game-aware and identifiable from actions alone.



\paragraph{Output data.}
All variants yield an offline dataset
\[
\mathcal D_{\text{off}}=\{(A_{1,t},A_{2,t})\}_{t=1}^{T},
\]
containing only observed actions.  P1 later trains a neural network to
approximate $p_\theta(A_2\mid A_1)$ using cross-entropy loss.



\pagebreak
\section{Experiment Design}

\paragraph{Game setup.}
We study a two-player zero sum
$\mathcal{A}_1=\{1,\dots,A_1\}$ for Player~1 (P1) and $\mathcal{A}_2=\{1,\dots,A_2\}$ for Player~2 (P2).
P1 receives payoff $R_1(a_1,a_2)$ and P2 receives $R_2(a_1,a_2)$ (in the zero-sum case, $R_2=-R_1$).

\paragraph{Offline data generation (fictitious-play-like).}
We generate an offline dataset $D_{\mathrm{off}}=\{(a_{1,t},a_{2,t})\}_{t=1}^{T}$ using a smoothed,
stochastic variant of fictitious play. The simulator maintains exponentially-smoothed beliefs over
action frequencies $FP_{1,t}\in\Delta(\mathcal{A}_1)$ and $FP_{2,t}\in\Delta(\mathcal{A}_2)$, initialized
uniformly. At each step $t$:
\begin{align}
a_2' &\sim FP_{2,t}, &
a_{1,t} &\sim \mathrm{SoftBR}_1(\cdot \mid a_2'),\\
a_1' &\sim FP_{1,t}, &
a_{2,t} &\sim \mathrm{SoftBR}_2(\cdot \mid a_1'),
\end{align}
where the soft best response is a temperature-scaled softmax over the relevant payoff slice:
\begin{align}
\mathrm{SoftBR}_1(a_1\mid a_2') &\propto \exp\!\Big(\tfrac{1}{\tau_1} R_1(a_1,a_2')\Big),\\
\mathrm{SoftBR}_2(a_2\mid a_1') &\propto \exp\!\Big(\tfrac{1}{\tau_2} R_2(a_1',a_2)\Big).
\end{align}
Beliefs are updated via exponential moving average with parameter $\alpha\in(0,1)$:
\begin{align}
FP_{1,t+1} &= \alpha FP_{1,t} + (1-\alpha)\, \mathbf{e}_{a_{1,t}},\\
FP_{2,t+1} &= \alpha FP_{2,t} + (1-\alpha)\, \mathbf{e}_{a_{2,t}},
\end{align}
where $\mathbf{e}_{a}$ denotes the one-hot vector for action $a$. We discard an initial burn-in
prefix to reduce transient effects.

\paragraph{Opponent modeling (offline supervised learning).}
From $D_{\mathrm{off}}$ we train P1's opponent model
\[
Q_{2,\theta}(a_2\mid a_1)
\]
using maximum likelihood (cross-entropy) on pairs $(a_1,a_2)$:
\begin{equation}
\mathcal{L}_2(\theta)=\mathbb{E}_{(a_1,a_2)\sim D}\big[-\log Q_{2,\theta}(a_2\mid a_1)\big].
\end{equation}
% ( we also fit $Q_{1,\phi}(a_1\mid a_2)$ for P2, but it is not used in the main adaptation experiment.)

\paragraph{Induced P1 policy via quantal response.}
Given $Q_{2,\theta}$, P1 computes the expected utility for each action
\begin{equation}
U_1(a_1)=\mathbb{E}_{a_2\sim Q_{2,\theta}(\cdot\mid a_1)}[R_1(a_1,a_2)]
=\sum_{a_2\in\mathcal{A}_2} Q_{2,\theta}(a_2\mid a_1)\,R_1(a_1,a_2),
\end{equation}
and selects actions according to a quantal (softmax) policy with inverse temperature $\beta$:
\begin{equation}
\pi_1(a_1)\propto \exp(\beta U_1(a_1)).
\end{equation}

\paragraph{Online adaptation with fixed P2 environment.}
We freeze P2 as a stochastic environment defined by the empirical conditional distribution extracted
from $D_{\mathrm{off}}$:
\begin{equation}
P2_{\mathrm{true}}(a_2\mid a_1)=
\frac{\#\{t:\ a_{1,t}=a_1,\ a_{2,t}=a_2\}}{\#\{t:\ a_{1,t}=a_1\}}.
\end{equation}
During online interaction, at each step $t$ we sample
\begin{equation}
a_{1,t}\sim \pi_1,\qquad a_{2,t}\sim P2_{\mathrm{true}}(\cdot\mid a_{1,t}),
\end{equation}
append $(a_{1,t},a_{2,t})$ to the online dataset $D_{\mathrm{on}}$, and periodically retrain
$Q_{2,\theta}$ on $D_{\mathrm{on}}$ (every $K$ steps). This produces a trajectory of models and induced
policies over time.

\paragraph{Reference Nash equilibrium.}
For the $2\times 2$ case we compute the mixed Nash equilibrium strategy $\pi_1^*$ analytically and
use it as a reference point. We quantify deviation from Nash using
\begin{equation}
D_{\mathrm{KL}}(\pi_1 \,\|\, \pi_1^*).
\end{equation}

\paragraph{Conditional vs.\ Unconditional Quantal Response Baselines.}
We study a two-player game with P1 actions $a_1\in\mathcal A_1$ and P2 actions $a_2\in\mathcal A_2$ and payoff $R_1(a_1,a_2)$ for P1. From offline data, we construct a fixed (frozen) conditional environment for P2:
\begin{equation}
P_{2,\mathrm{true}}(a_2\mid a_1),
\end{equation}
estimated via empirical counts.

\paragraph{Conditional quantal response (model-induced).}
Given an opponent model $Q_{2,\theta}(a_2\mid a_1)$ trained by maximum likelihood on pairs $(a_1,a_2)$, P1 computes the conditional expected utility
\begin{equation}
U_{\mathrm{cond}}(a_1)
\;=\;
\sum_{a_2\in\mathcal A_2} Q_{2,\theta}(a_2\mid a_1)\,R_1(a_1,a_2),
\end{equation}
and selects actions using a quantal (softmax) policy with inverse temperature $\beta>0$:
\begin{equation}
\pi_{\mathrm{cond}}(a_1)
\;=\;
\frac{\exp\big(\beta\,U_{\mathrm{cond}}(a_1)\big)}
{\sum_{a_1'\in\mathcal A_1}\exp\big(\beta\,U_{\mathrm{cond}}(a_1')\big)}.
\end{equation}
This policy is \emph{conditional} in the sense that the utilities depend on a different conditional opponent distribution for each $a_1$.

\vscomment{Here we do the following:
\begin{enumerate}
    \item If joint distribution of actions is $\rho(a_1,a_2)$, then we have the joint correlated QR to be 
    \begin{align*}
        \pi(a_1,a_2;\rho) & \propto \exp(\beta \rho(a_1,a_2) U_1(a_1,a_2))\\
        \pi(a_1,a_2;\rho) & \propto \exp(\beta \rho(a_1,a_2) U_2(a_1,a_2))\\
        \Rightarrow\  \pi(a_1,a_2;\rho) & \propto \exp(\beta \rho(a_1,a_2) (U_1(a_1,a_2)+U_2(a_1,a_2)))
    \end{align*}
    Therefore, 
    \begin{align*}
        \pi(a_1,a_2;\rho) & = \frac{\exp(\beta \rho(a_1,a_2) (U_1(a_1,a_2)+U_2(a_1,a_2)))}{\sum_{a_1^*,a_2^*}\exp(\beta \rho(a_1^*,a_2^*) (U_1(a_1^*,a_2^*)+U_2(a_1^*,a_2^*)))}
    \end{align*}
    \item Fixed point of above will be a correlated QRE.
\end{enumerate}
I am not sure that this works.
}

\azcomment{
\begin{align*}
F &: \Delta(A_1 \times A_2) \to \Delta(A_1 \times A_2), \\[6pt]
(F(\rho))(a_1,a_2)
&:= \frac{\exp\!\Bigl(
\beta\,\rho(a_1,a_2)
\bigl(U_1(a_1,a_2)+U_2(a_1,a_2)\bigr)
\Bigr)}
{\sum_{a_1',a_2'}
\exp\!\Bigl(
\beta\,\rho(a_1',a_2')
\bigl(U_1(a_1',a_2')+U_2(a_1',a_2')\bigr)
\Bigr)}, \\
\rho^\star &= F(\rho^\star).
\end{align*}
}

\vscomment{
Another attempt:
\begin{enumerate}
    \item Given joint distribution $\rho(a_1,a_2)$, then we obtain the conditional distribution of agent 2 given agent 1, $\rho_{2|1}(a_2|a_1)$, and the conditional distribution of agent 1 given agent 2, $\rho_{1|2}(a_1|a_2)$.
    \item Then, we have 
\end{enumerate}
}

\vscomment{The following reworkings of the CE definition could help in the generalization. In either case, the change of preferences per action becomes clear, and it is not immediate how to reconcile them easily for a QR type weighting.}

\vscomment{\textbf{First reworking:} we view $\rho(\cdot|a_1)$ as a distribution $\pi_{2|a_1}$ on $A_2$. Then, the CE condition (assuming full support) says: for all $a_1\in A_1$
\begin{align*}
    a_1 & \in \arg\max_{\tilde{a}_1\in A_1} \sum_{a_2} \pi_{2|a_1}(a_2) U_1(\tilde{a}_1,a_2) \\
    \Leftrightarrow\ \delta_{a_1} & \in \arg\max_{\pi_1\in \Delta(A_1)} \sum_{\tilde{a}_1, a_2} \pi_1(\tilde{a}_1) \pi_{2|a_1}(a_2) U_1(\tilde{a}_1,a_2)
\end{align*}
\textbf{Second reworking:} we view the utilities being changed by the action of each agent, i.e., for agent $1$ playing action $a_1$, the utility for action-pair $(\tilde{a}_1,a_2)$ is $\tilde{U}_{1,a_1}(\tilde{a}_1,a_2)=\rho(a_1,a_2) U_1(\tilde{a}_1,a_2)$. Then, the CE condition says: for all $a_1\in A_1$
\begin{align*}
    \delta_{a_1} & \in \arg\max_{\pi_1\in \Delta(A_1)} \sum_{\tilde{a}_1, a_2} \pi_1(\tilde{a}_1) \tilde{U}_{1,a_1}(\tilde{a}_1,a_2)
\end{align*}
This avoids issues with $\rho(a_1)=0$.}
%\\
%\textbf{Third reworking:} Given a CE $\rho(\cdot,\cdot)$, for 

\vscomment{In generalizing to quantal response, the best view would be to consider these as constraints on utility and then a minimization of the cost of the mixed strategy. Specifically, we will consider
\begin{align*}
    \min_{\rho(\cdot,\cdot) \in \Delta(A_1\otimes A_2)} & \sum_{(a_1,a_2)\in A_1 \otimes A_2} \rho(a_1,a_2) \log(\rho(a_1,a_2)) \\
    \text{subject to the following:} & \\
    \forall a_1\in A_1\ \sum_{a_2\in A_2} \rho(a_1,a_2) U_1(a_1,a_2) & \geq  \max_{\pi_1\in \Delta(A_1)} \sum_{\tilde{a}_1, a_2} \pi_1(\tilde{a}_1) \rho(a_1,a_2) U_1(\tilde{a}_1,a_2) -\gamma_{a_1} \\
    \forall a_2\in A_2\ \sum_{a_1\in A_1} \rho(a_1,a_2) U_2(a_1,a_2) & \geq  \max_{\pi_2\in \Delta(A_2)} \sum_{a_1, \tilde{a}_2} \pi_2(\tilde{a}_2) \rho(a_1,a_2) U_2(a_1,\tilde{a}_2) -\gamma_{a_2}
\end{align*}
for some prescribed vector $\gamma\geq 0$. If $\gamma=0$, then we have the set of CE that one is optimizing over (so, a refinement).}

\vscomment{The problem above is a convex program. Note that we have for $a_1\in A_1$
\begin{align*}
    \sum_{a_2\in A_2} \rho(a_1,a_2) U_1(a_1,a_2) & \geq  \max_{\pi_1\in \Delta(A_1)} \sum_{\tilde{a}_1, a_2} \pi_1(\tilde{a}_1) \rho(a_1,a_2) U_1(\tilde{a}_1,a_2) -\gamma_{a_1}\\
    \Leftrightarrow\ \sum_{a_2\in A_2} \rho(a_1,a_2) U_1(a_1,a_2) & \geq  \sum_{a_2\in A_2} \rho(a_1,a_2) U_1(\tilde{a}_1,a_2) -\gamma_{a_1}, \quad \forall \tilde{a}_1 \in A_1\setminus\{a_1\},
\end{align*}
which is a set of $|A_1|-1$ linear constraints. Hence, considering all actions and both agents, we have $|A_1|(|A_1|-1)+|A_2|(|A_2|-1)$ linear constraints; this is just like the conditions for a CE. Then, defining $\lambda_{a_i,\tilde{a}_i}$ as the Lagrange multiplier for each constraint, the equivalent problem is
\begin{align*}
    \min_{\rho(\cdot,\cdot) \in \Delta(A_1\otimes A_2)} & \sum_{(a_1,a_2)\in A_1 \otimes A_2} \rho(a_1,a_2) \log(\rho(a_1,a_2)) \\
    & \qquad \qquad + \rho(a_1,a_2) \Bigg( \sum_{\tilde{a}_1 \in A_1\setminus\{a_1\} }\lambda_{a_1,\tilde{a}_1} \big(U_1(\tilde{a}_1,a_2)-U_1(a_1,a_2)\big) \\
    & \qquad \qquad \qquad \qquad \qquad + \sum_{\tilde{a}_2 \in A_2\setminus\{a_2\} }\lambda_{a_2,\tilde{a}_2}\big(U_2(a_1,\tilde{a}_2)-U_2(a_1,a_2)\big)  \Bigg)
\end{align*}
Then, it is obvious that the solution is given by
\begin{align*}
    \rho(a_1,a_2) \propto e^{\sum_{\tilde{a}_1 \in A_1\setminus\{a_1\} }\lambda_{a_1,\tilde{a}_1} \big(U_1(a_1,a_2)-U_1(\tilde{a}_1,a_2)\big) + \sum_{\tilde{a}_2 \in A_2\setminus\{a_2\} }\lambda_{a_2,\tilde{a}_2}\big(U_2(a_1,a_2)-U_2(a_1,\tilde{a}_2)\big)}
\end{align*}
Thus, we can parameterize a correlated QRE by the $|A_1|(|A_1|-1)+|A_2|(|A_2|-1)$ non-negative numbers $\{\lambda_{a_i,\tilde{a}_i}\}_{i\in\{1,2\}, a_i\in A_i, \tilde{a}_i\in A_i\setminus\{a_i\}}$. Taking these numbers to $+\infty$ will yield a CE with the specific selection depending on the sequence used.}


\begin{theorem}[Existence]
Let $A_1$ and $A_2$ be finite action sets, let $U_1,U_2$ be bounded utility functions, and let $\gamma \ge 0$. Consider the optimization problem
\[
\min_{\rho \in \Delta(A_1 \times A_2)} \sum_{(a_1,a_2)\in A_1\times A_2} \rho(a_1,a_2)\log \rho(a_1,a_2)
\]
subject to the obedience constraints
\[
\sum_{a_2}\rho(a_1,a_2)\bigl(U_1(\tilde a_1,a_2)-U_1(a_1,a_2)\bigr)\le \gamma_{a_1},
\qquad \forall a_1\in A_1,\ \forall \tilde a_1\neq a_1,
\]
and
\[
\sum_{a_1}\rho(a_1,a_2)\bigl(U_2(a_1,\tilde a_2)-U_2(a_1,a_2)\bigr)\le \gamma_{a_2},
\qquad \forall a_2\in A_2,\ \forall \tilde a_2\neq a_2.
\]
Then this problem admits at least one minimizer.
\end{theorem}

\begin{proof}
Let $K_\gamma$ denote the feasible set. Since the game is finite, there exists a mixed Nash equilibrium $(\sigma_1,\sigma_2)$; the associated product distribution $\bar\rho(a_1,a_2)=\sigma_1(a_1)\sigma_2(a_2)$ satisfies all obedience constraints with slack at most $0$, hence belongs to $K_\gamma$ because $\gamma\ge 0$. Therefore $K_\gamma$ is nonempty. Moreover, $K_\gamma$ is a subset of the simplex $\Delta(A_1\times A_2)$, which is compact in finite dimensions, and each obedience constraint is linear in $\rho$, hence defines a closed half-space. It follows that $K_\gamma$ is a closed subset of a compact set, and is therefore compact. Finally, with the convention $0\log 0:=0$, the function $x\mapsto x\log x$ is continuous on $[0,1]$, so the objective $\rho\mapsto \sum_{(a_1,a_2)} \rho(a_1,a_2)\log \rho(a_1,a_2)$ is continuous on $K_\gamma$. By the Weierstrass theorem, a continuous function on a nonempty compact set attains its minimum. Hence the optimization problem admits a minimizer.
\end{proof}

\begin{theorem}[Uniqueness]
Let $A_1$ and $A_2$ be finite action sets, let $U_1,U_2$ be bounded utility functions, and let $\gamma \ge 0$. Consider the optimization problem
\[
\min_{\rho \in \Delta(A_1 \times A_2)} \sum_{(a_1,a_2)\in A_1\times A_2} \rho(a_1,a_2)\log \rho(a_1,a_2)
\]
subject to the obedience constraints
\[
\sum_{a_2}\rho(a_1,a_2)\bigl(U_1(\tilde a_1,a_2)-U_1(a_1,a_2)\bigr)\le \gamma_{a_1},
\qquad \forall a_1\in A_1,\ \forall \tilde a_1\neq a_1,
\]
and 
\[
\sum_{a_1}\rho(a_1,a_2)\bigl(U_2(a_1,\tilde a_2)-U_2(a_1,a_2)\bigr)\le \gamma_{a_2},
\qquad \forall a_2\in A_2,\ \forall \tilde a_2\neq a_2.
\]
Then the problem admits a unique minimizer.
\end{theorem}

\begin{proof}
Let $K_\gamma$ denote the feasible set. Since $\Delta(A_1\times A_2)$ is convex and each obedience constraint is linear in $\rho$, the set $K_\gamma$ is convex. Moreover, with the convention $0\log 0:=0$, the scalar function $x\mapsto x\log x$ is strictly convex on $[0,1]$, and therefore the objective
\[
F(\rho)=\sum_{(a_1,a_2)\in A_1\times A_2}\rho(a_1,a_2)\log \rho(a_1,a_2)
\]
is strictly convex on $\Delta(A_1\times A_2)$, hence on $K_\gamma$. Suppose for contradiction that there exist two distinct minimizers $\rho^\star,\tilde\rho^\star\in K_\gamma$. By convexity of $K_\gamma$, their midpoint $\bar\rho=\frac12(\rho^\star+\tilde\rho^\star)$ also lies in $K_\gamma$. Since $F$ is strictly convex and $\rho^\star\neq \tilde\rho^\star$, we have
\[
F(\bar\rho)<\frac12F(\rho^\star)+\frac12F(\tilde\rho^\star).
\]
But $\rho^\star$ and $\tilde\rho^\star$ are both minimizers, so $F(\rho^\star)=F(\tilde\rho^\star)$, and hence
\[
F(\bar\rho)<F(\rho^\star),
\]
contradicting the optimality of $\rho^\star$. Therefore the minimizer is unique.
\end{proof}



\pagebreak

\paragraph{Attempt 2}

Let $\rho \in \Delta(\mathcal A_1 \times \mathcal A_2)$ be a joint distribution over action pairs.


The marginals are
\begin{align}
\rho_1(a_1)
&:= \sum_{a_2 \in \mathcal A_2} \rho(a_1,a_2), 
\label{eq:marginal_p1} \\
\rho_2(a_2)
&:= \sum_{a_1 \in \mathcal A_1} \rho(a_1,a_2).
\label{eq:marginal_p2}
\end{align}

The induced conditionals are
\begin{align}
\rho_{2 \mid 1}(a_2 \mid a_1)
&:= \frac{\rho(a_1,a_2)}{\rho_1(a_1)},
\qquad \rho_1(a_1) > 0,
\label{eq:cond_p2_given_p1} \\
\rho_{1 \mid 2}(a_1 \mid a_2)
&:= \frac{\rho(a_1,a_2)}{\rho_2(a_2)},
\qquad \rho_2(a_2) > 0.
\label{eq:cond_p1_given_p2}
\end{align}


For Player~1, define the conditional value of switching from $a_1$ to $a_1'$ under $\rho$:
\begin{align}
V_1(a_1' \mid a_1; \rho)
&:= \sum_{a_2 \in \mathcal A_2}
\rho_{2 \mid 1}(a_2 \mid a_1)\,
R_1(a_1',a_2).
\label{eq:V1_def}
\end{align}

Similarly, for Player~2:
\begin{align}
V_2(a_2' \mid a_2; \rho)
&:= \sum_{a_1 \in \mathcal A_1}
\rho_{1 \mid 2}(a_1 \mid a_2)\,
R_2(a_1,a_2').
\label{eq:V2_def}
\end{align}

\paragraph{Correlated Equilibrium constraints}

We say that $\rho$ is a correlated equilibrium if
\begin{align}
V_1(a_1 \mid a_1; \rho)
&\ge
V_1(a_1' \mid a_1; \rho),
&&
\forall a_1 \text{ with } \rho_1(a_1) > 0,\ 
\forall a_1' \in \mathcal A_1,
\label{eq:ce_p1_cond}
\\
V_2(a_2 \mid a_2; \rho)
&\ge
V_2(a_2' \mid a_2; \rho),
&&
\forall a_2 \text{ with } \rho_2(a_2) > 0,\ 
\forall a_2' \in \mathcal A_2.
\label{eq:ce_p2_cond}
\end{align}

If $\rho_1(a_1)=0$ or $\rho_2(a_2)=0$?

\paragraph{No conditional joint form}

Multiplying \eqref{eq:ce_p1_cond} by $\rho_1(a_1)$ and
\eqref{eq:ce_p2_cond} by $\rho_2(a_2)$:

\begin{align}
\sum_{a_2 \in \mathcal A_2}
\rho(a_1,a_2)\,
R_1(a_1,a_2)
&\ge
\sum_{a_2 \in \mathcal A_2}
\rho(a_1,a_2)\,
R_1(a_1',a_2),
\notag \\
&\qquad
\forall a_1,a_1' \in \mathcal A_1,
\label{eq:ce_p1_joint}
\\[4pt]
\sum_{a_1 \in \mathcal A_1}
\rho(a_1,a_2)\,
R_2(a_1,a_2)
&\ge
\sum_{a_1 \in \mathcal A_1}
\rho(a_1,a_2)\,
R_2(a_1,a_2'),
\notag \\
&\qquad
\forall a_2,a_2' \in \mathcal A_2.
\label{eq:ce_p2_joint}
\end{align}



Equivalently, for any deviation maps
$\phi_1:\mathcal A_1 \to \mathcal A_1$ and
$\phi_2:\mathcal A_2 \to \mathcal A_2$:

\begin{align}
\sum_{a_1,a_2}
\rho(a_1,a_2)\,
R_1(a_1,a_2)
&\ge
\sum_{a_1,a_2}
\rho(a_1,a_2)\,
R_1(\phi_1(a_1),a_2),
\label{eq:ce_swap_p1}
\\
\sum_{a_1,a_2}
\rho(a_1,a_2)\,
R_2(a_1,a_2)
&\ge
\sum_{a_1,a_2}
\rho(a_1,a_2)\,
R_2(a_1,\phi_2(a_2)).
\label{eq:ce_swap_p2}
\end{align}


Given an empirical joint $\hat\rho$, define
\begin{align}
\mathrm{CERegret}_1(\hat\rho)
&:=
\max_{a_1,a_1'}
\sum_{a_2}
\hat\rho(a_1,a_2)
\bigl(
R_1(a_1',a_2) - R_1(a_1,a_2)
\bigr),
\label{eq:ce_regret_1}
\end{align}
and analogously $\mathrm{CERegret}_2(\hat\rho)$.  
We have $\hat\rho$ is a CE iff both regrets are $\le 0$.



\pagebreak

\paragraph{Unconditional quantal response baseline }
Standard quantal response assumes P1 responds to a \emph{single} fixed mixed strategy of P2, i.e., a distribution over $a_2$ that does not condition on $a_1$.
Since our frozen environment is conditional, we form an unconditional P2 mixture by choosing a reference distribution $\rho(a_1)$ over P1 actions and marginalizing:
\begin{equation}\label{eq:player2_ms}
\bar P^{\,\rho}_2(a_2)
\;=\;
\sum_{a_1\in\mathcal A_1} \rho(a_1)\,P_{2,\mathrm{true}}(a_2\mid a_1).
\end{equation}
\vscomment{\eqref{eq:player2_ms} gives a mixed strategy for player 2 based on player 1's strategy $\rho$ and model of player 2 $P_{2,\mathrm{true}}$.}
We then define the \emph{unconditional} expected utility and the corresponding quantal-response policy:
\begin{equation}
U_{\mathrm{uncond}}^{\rho}(a_1)
\;=\;
\sum_{a_2\in\mathcal A_2} \bar P^{\,\rho}_2(a_2)\,R_1(a_1,a_2),
\end{equation}
\begin{equation}\label{eq:player1_qr}
\qquad
\pi_{\mathrm{uncond}}^{\rho}(a_1)
\;=\;
\frac{\exp\big(\beta\,U_{\mathrm{uncond}}^{\rho}(a_1)\big)}
{\sum_{a_1'\in\mathcal A_1}\exp\big(\beta\,U_{\mathrm{uncond}}^{\rho}(a_1')\big)}.
\end{equation}
\vscomment{\eqref{eq:player1_qr} gives player 1's quantal response to estimated mixed strategy of player 2.}
\vscomment{One possibility \eqref{eq:player2_ms}-\eqref{eq:player1_qr} takes $\rho_1$ produces $\hat{\rho}_2$ and $\pi_1(\rho_1)$ using $P_{2,true}$ and $U_1$. Player 2 does the same: takes $\rho_2$ produces $\hat{\rho}_1$ and $\pi_2(\rho_2)$ using $P_{1,true}$ and $U_2$. If $\rho_i=\pi_i(\rho_i)=\hat{\rho}_i$ for $i=1,2$, then equilibrium.}

\paragraph{Choice of reference distribution.}
In our implementation, we use the \emph{empirical} reference distribution from the offline dataset,
\begin{equation}
\rho_{\mathrm{emp}}(a_1)
\;=\;
\frac{\#\{t:\,a_{1,t}=a_1\}}{\sum_{a_1'\in\mathcal A_1}\#\{t:\,a_{1,t}=a_1'\}},
\end{equation}
so that $\bar P_2^{\,\rho_{\mathrm{emp}}}$ matches the overall marginal P2 behavior induced by the offline action frequencies of P1.

can also use the uniform reference $\rho_{\mathrm{unif}}(a_1)=1/|\mathcal A_1|$.


\subsection{Correlated Quantal Response Equilibrium (CQRE)}
\label{sec:cqre}

% \paragraph{Motivation.}
% In the conditional-QR setting, the natural equilibrium object is not just a pair of independent mixed
% strategies, but a \emph{joint} distribution over action pairs. This mirrors correlated equilibrium (CE),
% except that agents respond \emph{quantly} (softly) rather than best-responding exactly.

\paragraph{Setup (mediated play).}
Let $\mu \in \Delta(\mathcal A_1 \times \mathcal A_2)$ be a joint distribution over \emph{recommendations}
$(r_1,r_2)$. A mediator draws $(r_1,r_2)\sim \mu$ and privately recommends $r_i$ to player $i$.
Each player uses a \emph{response kernel}
\[
g_1(\cdot \mid r_1)\in \Delta(\mathcal A_1),\qquad
g_2(\cdot \mid r_2)\in \Delta(\mathcal A_2),
\]
so the realized actions $(a_1,a_2)$ may differ from the recommendations $(r_1,r_2)$.

\paragraph{Induced conditional beliefs over realized opponent actions.}
Given $\mu$ and $(g_1,g_2)$, the distribution of P2's \emph{realized} action conditional on P1's
recommendation $r_1$ is
\begin{equation}
\tilde P_2^{\mu,g}(a_2 \mid r_1)
\;=\;
\sum_{r_2 \in \mathcal A_2} \mu(r_2 \mid r_1)\, g_2(a_2 \mid r_2),
\label{eq:cqre_induced_P2}
\end{equation}
and symmetrically the distribution of P1's realized action conditional on P2's recommendation $r_2$ is
\begin{equation}
\tilde P_1^{\mu,g}(a_1 \mid r_2)
\;=\;
\sum_{r_1 \in \mathcal A_1} \mu(r_1 \mid r_2)\, g_1(a_1 \mid r_1).
\label{eq:cqre_induced_P1}
\end{equation}

\paragraph{Recommendation-conditioned expected utilities.}
For each recommendation $r_1$, P1 evaluates choosing action $a_1$ using the induced conditional in
\eqref{eq:cqre_induced_P2}:
\begin{equation}
EU_1^{\mu,g}(a_1 \mid r_1)
\;=\;
\sum_{a_2 \in \mathcal A_2} \tilde P_2^{\mu,g}(a_2 \mid r_1)\, R_1(a_1,a_2).
\label{eq:cqre_EU1}
\end{equation}
Similarly, for each recommendation $r_2$, P2 evaluates choosing $a_2$ via
\begin{equation}
EU_2^{\mu,g}(a_2 \mid r_2)
\;=\;
\sum_{a_1 \in \mathcal A_1} \tilde P_1^{\mu,g}(a_1 \mid r_2)\, R_2(a_1,a_2).
\label{eq:cqre_EU2}
\end{equation}

\paragraph{Quantal response to recommendations.}
Fix inverse temperatures $\beta_1,\beta_2>0$. The response kernels are defined by the logit rule:
\begin{align}
g_1(a_1 \mid r_1)
&=
\frac{\exp\!\big(\beta_1\,EU_1^{\mu,g}(a_1 \mid r_1)\big)}
{\sum_{a_1'\in\mathcal A_1}\exp\!\big(\beta_1\,EU_1^{\mu,g}(a_1' \mid r_1)\big)},
\label{eq:cqre_logit1}\\
g_2(a_2 \mid r_2)
&=
\frac{\exp\!\big(\beta_2\,EU_2^{\mu,g}(a_2 \mid r_2)\big)}
{\sum_{a_2'\in\mathcal A_2}\exp\!\big(\beta_2\,EU_2^{\mu,g}(a_2' \mid r_2)\big)}.
\label{eq:cqre_logit2}
\end{align}

\paragraph{Consistency (fixed point in the joint distribution).}
The mediator's recommendation distribution $\mu$ should coincide with the \emph{distribution of realized play}
induced by drawing recommendations from $\mu$ and then responding via $(g_1,g_2)$:
\begin{equation}
\mu(a_1,a_2)
\;=\;
\sum_{r_1\in\mathcal A_1}\sum_{r_2\in\mathcal A_2}
\mu(r_1,r_2)\, g_1(a_1 \mid r_1)\, g_2(a_2 \mid r_2),
\qquad \forall (a_1,a_2)\in\mathcal A_1\times\mathcal A_2.
\label{eq:cqre_consistency}
\end{equation}

\paragraph{Definition (CQRE).}
A \emph{correlated quantal response equilibrium} is a triple $(\mu,g_1,g_2)$ such that
(i) $(g_1,g_2)$ satisfy the logit best-response conditions \eqref{eq:cqre_logit1}--\eqref{eq:cqre_logit2}
with expected utilities \eqref{eq:cqre_EU1}--\eqref{eq:cqre_EU2} induced by $\mu$ through
\eqref{eq:cqre_induced_P2}--\eqref{eq:cqre_induced_P1}, and (ii) $\mu$ satisfies the consistency condition
\eqref{eq:cqre_consistency}.

\paragraph{Relation to familiar notions (informal).}
When $\beta_i\to\infty$, the logit responses concentrate on best responses, and CQRE approaches a correlated
equilibrium (CE). If $\mu(r_2\mid r_1)$ does not depend on $r_1$ (no correlation/information), CQRE reduces
to the standard quantal-response logic against a single mixed opponent distribution.

\paragraph{Connection to conditional-QR opponent modeling.}
the learned conditional model $Q_{2,\theta}(a_2\mid a_1)$ can be interpreted as an approximation to the
equilibrium-induced conditional $\tilde P_2^{\mu,g}(a_2\mid r_1)$ evaluated at $r_1=a_1$. In CQRE, however,
both players' conditionals must be mutually consistent through the fixed-point condition \eqref{eq:cqre_consistency},
rather than treating P2 as a frozen conditional environment.


\paragraph{Game.}
We consider a $2\times 2$ zero-sum game with a unique interior mixed Nash equilibrium (NE).
Player~1 has actions $\{A1,A2\}$ and Player~2 has actions $\{B1,B2\}$.
Let $R_1\in\mathbb{R}^{2\times 2}$ denote Player~1's payoff matrix (rows correspond to $A1/A2$, columns to $B1/B2$), and $R_2=-R_1$ denote Player~2's payoff matrix:
\[
R_1 =
\begin{bmatrix}
-2 & -1\\
0 & -2
\end{bmatrix},
\qquad
R_2 = -R_1 =
\begin{bmatrix}
2 & 1\\
0 & 2
\end{bmatrix}.
\]
The mixed Nash equilibrium is interior and unique, given by
\[
\pi_1^*(A1)=\frac{2}{3},\quad \pi_1^*(A2)=\frac{1}{3},
\qquad
\pi_2^*(B1)=\frac{1}{3},\quad \pi_2^*(B2)=\frac{2}{3}.
\]







\paragraph{What the comparison measures.}
We compare the learned \emph{conditional} policy $\pi_{\mathrm{cond}}$ against the \emph{unconditional} baseline $\pi_{\mathrm{uncond}}^{\rho}$ (and optionally their KL divergence) to quantify how much P1's behavior is driven by action-dependent opponent modeling versus responding to a single aggregated P2 mixture.






% \section{Visualization Summary}

% We visualize learning and adaptation using four plots evaluated at each retraining checkpoint:
% \begin{enumerate}
% \item \textbf{Utility evolution:} $U_1(A1)$ and $U_1(A2)$ over online steps, where
% $U_1(a_1)=\sum_{a_2}Q_{2,\theta}(a_2\mid a_1)R_1(a_1,a_2)$.
% \item \textbf{Opponent model accuracy:} $Q_{2,\theta}(B1\mid A1)$ and $Q_{2,\theta}(B1\mid A2)$
% (solid) compared against the empirical environment
% $P2_{\mathrm{true}}(B1\mid A1)$ and $P2_{\mathrm{true}}(B1\mid A2)$ (dashed).
% \item \textbf{Policy vs.\ Nash:} the induced policy component $\pi_1(A1)$ (solid) compared to the
% mixed Nash equilibrium probability $\pi_1^*(A1)$ (dashed).
% \item \textbf{Distance to Nash:} $D_{\mathrm{KL}}(\pi_1\|\pi_1^*)$ over time, measuring how far the
% induced policy is from the Nash reference.
% \end{enumerate}

% \paragraph{Interpretation guide.}
% If $Q_{2,\theta}$ tracks $P2_{\mathrm{true}}$, then the opponent model is learning the (frozen)
% environment. If $P2_{\mathrm{true}}$ differs from P2's Nash strategy, the induced $\pi_1$ will generally
% converge toward a (soft) best response to $P2_{\mathrm{true}}$, and may remain far from $\pi_1^*$,
% yielding a persistently nonzero $D_{\mathrm{KL}}(\pi_1\|\pi_1^*)$.















\subsection{Correlated Quantal Response Equilibrium (CQRE)}
\label{sec:cqre}

\paragraph{Setup (mediated play).}
Let $\psi \in \Delta(\mathcal A_1 \times \mathcal A_2)$ be a joint distribution over \emph{recommendations}
$(r_1,r_2)$. A mediator draws $(r_1,r_2)\sim \psi$ and privately recommends $r_i$ to player $i$.
Each player uses a \emph{response kernel}
\[
g_1(\cdot \mid r_1)\in \Delta(\mathcal A_1),\qquad
g_2(\cdot \mid r_2)\in \Delta(\mathcal A_2),
\]
so the realized actions $(a_1,a_2)$ may differ from the recommendations $(r_1,r_2)$.

\paragraph{Induced conditional beliefs over realized opponent actions.}
Given $\psi$ and $(g_1,g_2)$, the distribution of P2's \emph{realized} action conditional on P1's
recommendation $r_1$ is
\begin{equation}
\tilde P_2^{\psi,g}(a_2 \mid r_1)
\;=\;
\sum_{r_2 \in \mathcal A_2} \psi(r_2 \mid r_1)\, g_2(a_2 \mid r_2),
\label{eq:cqre_induced_P2_new}
\end{equation}
and symmetrically the distribution of P1's realized action conditional on P2's recommendation $r_2$ is
\begin{equation}
\tilde P_1^{\psi,g}(a_1 \mid r_2)
\;=\;
\sum_{r_1 \in \mathcal A_1} \psi(r_1 \mid r_2)\, g_1(a_1 \mid r_1).
\label{eq:cqre_induced_P1_new}
\end{equation}

\paragraph{Recommendation-conditioned expected utilities.}
For each recommendation $r_1$, P1 evaluates choosing action $a_1$ using the induced conditional in
\eqref{eq:cqre_induced_P2_new}:
\begin{equation}
EU_1^{\psi,g}(a_1 \mid r_1)
\;=\;
\sum_{a_2 \in \mathcal A_2} \tilde P_2^{\psi,g}(a_2 \mid r_1)\, R_1(a_1,a_2).
\label{eq:cqre_EU1_new}
\end{equation}
Similarly, for each recommendation $r_2$, P2 evaluates choosing $a_2$ via
\begin{equation}
EU_2^{\psi,g}(a_2 \mid r_2)
\;=\;
\sum_{a_1 \in \mathcal A_1} \tilde P_1^{\psi,g}(a_1 \mid r_2)\, R_2(a_1,a_2).
\label{eq:cqre_EU2_new}
\end{equation}

\paragraph{Quantal response to recommendations.}
Fix inverse temperatures $\beta_1,\beta_2>0$. The response kernels are defined by the logit rule:
\begin{align}
g_1(a_1 \mid r_1)
&=
\frac{\exp\!\big(\beta_1\,EU_1^{\psi,g}(a_1 \mid r_1)\big)}
{\sum_{a_1'\in\mathcal A_1}\exp\!\big(\beta_1\,EU_1^{\psi,g}(a_1' \mid r_1)\big)},
\label{eq:cqre_logit1_new}\\
g_2(a_2 \mid r_2)
&=
\frac{\exp\!\big(\beta_2\,EU_2^{\psi,g}(a_2 \mid r_2)\big)}
{\sum_{a_2'\in\mathcal A_2}\exp\!\big(\beta_2\,EU_2^{\psi,g}(a_2' \mid r_2)\big)}.
\label{eq:cqre_logit2_new}
\end{align}

\paragraph{Consistency (fixed point in the joint distribution).}
Let $\mu^{\psi,g}\in \Delta(\mathcal A_1\times \mathcal A_2)$ denote the \emph{distribution of realized play}
induced by drawing recommendations from $\psi$ and then responding via $(g_1,g_2)$:
\begin{equation}
\mu^{\psi,g}(a_1,a_2)
\;=\;
\sum_{r_1\in\mathcal A_1}\sum_{r_2\in\mathcal A_2}
\psi(r_1,r_2)\, g_1(a_1 \mid r_1)\, g_2(a_2 \mid r_2),
\qquad \forall (a_1,a_2)\in\mathcal A_1\times\mathcal A_2.
\label{eq:cqre_induced_mu_new}
\end{equation}
The mediator's recommendation distribution $\psi$ must coincide with the induced realized-play distribution:
\begin{equation}
\psi(a_1,a_2) \;=\; \mu^{\psi,g}(a_1,a_2),
\qquad \forall (a_1,a_2)\in\mathcal A_1\times\mathcal A_2.
\label{eq:cqre_consistency_new}
\end{equation}
Equivalently, combining \eqref{eq:cqre_induced_mu_new} and \eqref{eq:cqre_consistency_new} yields the
fixed-point form
\begin{equation}
\psi(a_1,a_2)
\;=\;
\sum_{r_1\in\mathcal A_1}\sum_{r_2\in\mathcal A_2}
\psi(r_1,r_2)\, g_1(a_1 \mid r_1)\, g_2(a_2 \mid r_2).
\label{eq:cqre_fixed_point_new}
\end{equation}

\paragraph{Definition (CQRE).}
A \emph{correlated quantal response equilibrium} is a triple $(\psi,g_1,g_2)$ such that
(i) $(g_1,g_2)$ satisfy the logit best-response conditions \eqref{eq:cqre_logit1_new}--\eqref{eq:cqre_logit2_new}
with expected utilities \eqref{eq:cqre_EU1_new}--\eqref{eq:cqre_EU2_new} induced by $\psi$ through
\eqref{eq:cqre_induced_P2_new}--\eqref{eq:cqre_induced_P1_new}, and (ii) $\psi$ satisfies the consistency
condition \eqref{eq:cqre_consistency_new} (equivalently \eqref{eq:cqre_fixed_point_new}).

\paragraph{Relation to familiar notions.}
When $\beta_i\to\infty$, the logit responses concentrate on best responses, and CQRE approaches a correlated
equilibrium (CE). If $\psi(r_2\mid r_1)$ does not depend on $r_1$ (no correlation/information), CQRE reduces
to the standard quantal-response logic against a single mixed opponent distribution.

\paragraph{Connection to conditional-QR opponent modeling.}
The learned conditional model $Q_{2,\theta}(a_2\mid a_1)$ can be interpreted as an approximation to the
equilibrium-induced conditional $\tilde P_2^{\psi,g}(a_2\mid r_1)$ evaluated at $r_1=a_1$. In CQRE, however,
both players' conditionals must be mutually consistent through the fixed-point condition
\eqref{eq:cqre_consistency_new}, rather than treating P2 as a frozen conditional environment.


% Requires (in preamble):
% \usepackage{amsthm,amsmath,amssymb}
% \newtheorem{definition}{Definition}
% \newtheorem{proposition}{Proposition}

\subsection{Signal-Conditioned Logit Quantal Response Equilibrium}
\label{sec:sclqre}

We formalize an equilibrium concept that combines an Aumann-style information structure
(players condition only on what they observe) with logit (softmax) best responses.

\paragraph{Information structure.}
Fix a finite normal-form game $\Gamma=(N,\{A_i\}_{i\in N},\{u_i\}_{i\in N})$.
An information structure is a tuple $(\Omega,\mu,\{P_i\}_{i\in N})$ where $\Omega$ is a finite set of worlds,
$\mu\in\Delta(\Omega)$ is a common prior, and $P_i$ is a partition of $\Omega$ representing player $i$'s information.
For each $\omega\in\Omega$, let $C_i(\omega)\in P_i$ denote the unique cell containing $\omega$; player $i$ observes
$C_i=C_i(\omega)$ rather than $\omega$ itself. The vector $(C_1(\omega),\dots,C_N(\omega))$ is generally correlated
under $\mu$.

For any cell $C_i\in P_i$ with $\mu(C_i)>0$, define player $i$'s posterior belief as
\begin{equation}
b_i(\omega\mid C_i)\;:=\;\frac{\mu(\omega)\mathbf{1}\{\omega\in C_i\}}{\mu(C_i)}.
\label{eq:posterior_belief}
\end{equation}

\paragraph{Policies.}
A (mixed) behavioral policy for player $i$ is a map
\begin{equation}
\pi_i: P_i \to \Delta(A_i),
\label{eq:policy_pi}
\end{equation}
i.e., an action distribution chosen as a function of the observed information cell.
Given a world $\omega$, opponents act according to $\pi_j(\cdot\mid C_j(\omega))$.

Given $\pi_{-i}$, define the interim value of playing $a_i\in A_i$ upon observing $C_i\in P_i$ as
\begin{align}
V_i(a_i\mid C_i;\pi_{-i})
&:=\mathbb{E}_{\omega\sim b_i(\cdot\mid C_i)}
\Big[
\mathbb{E}_{a_{-i}\sim \prod_{j\neq i}\pi_j(\cdot\mid C_j(\omega))}
\big[u_i(a_i,a_{-i})\big]
\Big].
\label{eq:interim_value_V}
\end{align}
me
If only 2 players:
\begin{align}
V_1(a_1 \mid C_1;\pi_2)
&=\mathbb{E}_{\omega\sim b_1(\cdot\mid C_1)}
\Big[
\mathbb{E}_{a_2\sim \pi_2(\cdot\mid C_2(\omega))}\; u_1(a_1,a_2)
\Big], \\
V_2(a_2 \mid C_2;\pi_1)
&=\mathbb{E}_{\omega\sim b_2(\cdot\mid C_2)}
\Big[
\mathbb{E}_{a_1\sim \pi_1(\cdot\mid C_1(\omega))}\; u_2(a_1,a_2)
\Big].
\end{align}

\begin{definition}[Signal-Conditioned Logit-QRE (SC-LQRE)]
\label{def:sclqre}
Fix inverse-temperature (rationality) parameters $\lambda_i\ge 0$.
A policy profile $\pi=(\pi_i)_{i\in N}$ with $\pi_i:P_i\to\Delta(A_i)$ is a
\emph{signal-conditioned logit quantal response equilibrium} if for every player $i$ and every cell
$C_i\in P_i$ with $\mu(C_i)>0$,
\begin{equation}
\pi_i(a_i\mid C_i)
\;=\;
\frac{\exp\!\big(\lambda_i\,V_i(a_i\mid C_i;\pi_{-i})\big)}
{\sum_{a_i'\in A_i}\exp\!\big(\lambda_i\,V_i(a_i'\mid C_i;\pi_{-i})\big)}
\qquad\forall a_i\in A_i.
\label{eq:sclqre_softmax_pi}
\end{equation}
\end{definition}

\paragraph{Interpretation.}
Equation~\eqref{eq:sclqre_softmax_pi} says that within each information cell $C_i$, player $i$ plays a soft best response:
actions with larger interim value~\eqref{eq:interim_value_V} receive exponentially larger probability.
As $\lambda_i\to 0$, $\pi_i(\cdot\mid C_i)$ approaches uniform randomization; as $\lambda_i\to\infty$, it concentrates
on (cell-wise) best responses.

\begin{proposition}[Existence in the finite case]
\label{prop:existence_sclqre}
If $\Omega$ and all action sets $A_i$ are finite, then an SC-LQRE exists.
\end{proposition}

\noindent\emph{Proof.}
The policy space $\prod_i\prod_{C_i\in P_i}\Delta(A_i)$ is compact and convex.
The logit-response map defined by~\eqref{eq:sclqre_softmax_pi} is continuous, hence has a fixed point by Brouwer's theorem.







\end{document}
