# Supplementary material for: Correlated Quantal Response Equilibrium: A New Equilibrium Notion for Human-AI Strategic Interactions
Source: arXiv:2610.29020 source file (2026-10-21)
Supplement: Supplementary file 3 [file main-rj.tex]

\documentclass[11pt]{article}

% Language setting
% Replace `english' with e.g. `spanish' to change the document language
\usepackage[english]{babel} 
\usepackage{fullpage}
\usepackage[numbers,sort,compress]{natbib}

\newtheorem{theorem}{Theorem}[section]
\newtheorem{corollary}{Corollary}[theorem]
\newtheorem{lemma}[theorem]{Lemma}

% Set page size and margins
% Replace `letterpaper' with `a4paper' for UK/EU standard size
\usepackage[letterpaper,top=1in,bottom=1in,left=1in,right=1in,marginparwidth=1.75cm]{geometry}

% Useful packages
\usepackage{amsmath,amsthm,amstext,amsfonts,amssymb,mathrsfs}
\usepackage{graphicx}
\usepackage[colorlinks=true, allcolors=blue]{hyperref}
\usepackage{wrapfig}

\usepackage[most]{tcolorbox}
\usepackage[tikz]{mdframed}
\mdfsetup{outerlinewidth=1pt,innerlinewidth=0pt , outerlinecolor=black, roundcorner=2pt }	

% \mdfdefinestyle{MyFrame}{%
%     linecolor=black,
%     outerlinewidth=2pt,
%     %roundcorner=20pt,
%     innertopmargin=4pt,
%     innerbottommargin=4pt,
%     innerrightmargin=4pt,
%     innerleftmargin=4pt,
%         leftmargin = 4pt,
%         rightmargin = 4pt
%     %backgroundcolor=gray!50!white}
%         }
      

\title{\bf\sf A Theory of Learnable Equilibria}
\author{\bf\sf Rahul Jain\\
%\bf\sf USC Center for Autonomy and AI
}
\date{\today}

\begin{document}
\maketitle

\section{\bf\sf Introduction}

Standard solution concepts in game theory such as Nash equilibria, correlated equilibria, rational expectations(?), and their sequential and perfected variants are computationally intractable to compute, i.e., even when  the game model is known, it is PSPACE-hard to be able to complete even Nash equilibrium in matrix games [Papadimitrou, et al]. And yet, markets routinely equilibrate. Participants in auctions routinely find outcomes or “equilibria”, even when the mechanisms do not implement dominant strategy equilibria. When the model (payoffs, and transition dynamics models, when the game is sequential) is unknown, and other players are also trying to “learn” at the same time, the question is what “outcomes” (which do happen in real world settings) are they converging to. We will call such outcomes of multiplayer games as “learnable equilibria”. The question is how to define them so that they have some predictive power, and not just descriptive utility. We will  distinguish between “reinforcement learning”, i.e., learning of the game model 
(payoff functions and the transition dynamic model) when say the strategy of the other players is known), and “strategic learning”, i.e., learning of the strategy of the other player, i.e., learning the best response to the other players’ learning strategy when the game model is known. Of course, in practical settings both the game model and the learning strategy used by the other players is unknown. We refer to this as `strategic reinforcement learning’ (SRL).

In this proposal, we first propose models of behavior for players that are sufficiently general  to capture learning by agents in almost all settings. Agents could be autonomous or semi-autonomous. We then propose a general notion of “learnable equilibria”. Specifically, we show that BLAH fits the definition of such solution concepts. We then establish conditions for existence of such “learnable equilibria” in general settings. We then present learning algorithms that converge to such `learnable equilibria’. We then consider the poacher-law enforcement setting data from Africa, and show how computing `learnable equilibria’ of the game can be used to predict the next actions the poachers.

We now present a theory of learnable equilibria wherein each learning agent models the strategy of the other players, and learns the parameters of such a model over repeated interactions.


\section{\bf\sf Basic Idea: Static and Repeated Games of Full Information}

Consider a simple matrix game with two players (denoted $1, 2$), strategy spaces $A_i, A_j$, and payoff functions $u_i, u_j$. For now, we will assume all information is \textit{common knowledge}.

\subsection{\bf\sf Models of Behavior}

 The core of our approach relies on modeling strategic behavior of the other players. With such models, the decision making problem for each agent is akin to a single agent’s learning problem which can be solved, for example, by the successful and scalable approach for deep learning. Our initial focus will only be on first-order beliefs, i.e., each agent models the strategic behavior of each of the other players, without taking into account that other players also are building similar behavioral models for it for use in their decision-making. Such behavioral models could be as parametric forms of the strategies, particularly useful when access to payoffs of the other players is not available. We can also use non-parametric models such as DNNs and even transformers, if memory is needed to be incorporated.  Similarly, parametric forms of value functions could also be used as behavior models of other agents in case access to payoffs is available. We could also do both which would be helpful in designing Actor-Critic-style learning algorithms. 

A \textit{Nash equilibrium} of the game is $(a_1^*,a_2^*)$ if
\[
a_i^* \in \arg\max_{a_i} u_i(a_i, a_{-i}^*), ~\forall i.
\]
Denote \textit{best responses} by $\phi_i(a_{-i}) = \arg\max_a u_i(a, a_{-i}).$
The Nash equilibrium can also be written as
\[
a_i^* = \phi_i(a_{-i}^*),~\text{and}~
a_{-i}^* = \phi_{-i}(a_{i}^*).
\]
Now, let us parametrize the best response $\phi_i$ by $\theta_i$, i.e., $\phi_i \approx \phi_i^{\theta_i}, \theta_i \in \Theta$. We will call these \textit{behavioral best responses}. These parameteric functions could even be `non-parametric' models such as neural networks, where the paremeters are its weights. Then, given this ``behavioral model" for the other player, each player's decision problem becomes
\[
\tilde{a}_i = \arg \max_{a_i} u_i(a_i,\phi_{-i}^{\theta_{-i}}(a_i)).
\]
The parameters $\theta = (\theta_i, \theta_{-i})$ models the best response of the other player. 

\subsubsection{Modeling $k$-level belief systems}

For simplicity, we only consider two players. Let $\phi_{i}^{\theta_{i}^l}$ denote player $i$'s best response to player $-i$'s with parameters $\theta_{i}^l$ at level $l$. Then, player 2's best response at level 2 is:
\[
\Phi_{2}^{\theta_{2:2}^{2:1}}(a_1)=\phi_{2}^{\theta_{2}^2}(\phi_{1}^{\theta_{1}^1}(\phi_{2}^{\theta_{2}^1}(a_1))),
\]
where $\theta_{2:2}^{2:1} = (\theta_2^2,\theta_2^1,\theta_1^1)$. Similarly, player 1's best response at level 2 is:
\[
\Phi_{1}^{\vartheta_{1:1}^{2:1}}(a_1)=\phi_{1}^{\vartheta_{1}^2}(\phi_{2}^{\vartheta_{2}^1}(\phi_{1}^{\vartheta_{1}^1}(a_1))),
\]
where $\vartheta_{1:1}^{2:1} = (\vartheta_2^2,\vartheta_2^1,\vartheta_1^1)$. In general, denote $\theta_{i:i}^{k:1} = (\theta_i^k,\theta_{-i}^{k-1},\cdots,\theta_i^1)$, and respectively for $\vartheta_{i:i}^{k:1}$.

Thus, player 1's belief about level $k$ best response of player 2 is given by $\Phi_{2}^{\theta_{2:2}^{k:1}}$. Similarly, Player 2's belief about level 2 best response of player 1 is given by $\Phi_{1}^{\vartheta_{1:1}^{k:1}}$.

Thus, for any finite-level belief systems, there is no loss of generality in assuming a form $\Phi_i^{\theta_i}$ as a model for player $i$ best response by player $-i$. In fact, if such models are non-parametric, they should be able to model even infinitely-recursive belief systems.

\subsection{\bf\sf Learnable Solution Concepts}

%A key question is what are relevant notions of solution concepts or equilibrium for strategic learning. Clearly, it is a folly to consider classical solution concepts based on Nash equilbrium because we already know that even in simple settings there exist no learning algorithm that converge to it. A candidate is quantal response equilibrium, an equilibrium notion with bounded rationality. A specific example of it is logic equilibrium wherein players choose their mixed strategies according to logic function with expected utility. This resonates with similar successful approaches in online learning, e.g., the EXP3 algorithm.  The notion has been extended to dynamic games. The notion has been shown to successfully explain strategic behavior in some real-world games. Unfortunately, there can be a loss of information due to the mean-field approach. Another candidate is what we call `learnable equilbria’ where each agent uses a first-order model of the strategic behavior of the other agents. This is quite close to the practical approach used in AI systems such as AlphaGo, MuZero, etc. Other relevant notions to consider, particularly for incomplete information are concepts such as multiselves equilibrium, self-confirming equilibrium, etc. 

Let us consider parametrized mean payoff functions $\bar{u}_i(\pi_i,\pi_{-i},\theta_i)$.  $\theta_i$ are private information, and let $\hat{\theta}_i$ denote estimates of it by the other player. Then, we say that mixed strategies and beliefs $((\pi_1^*,\hat{\theta}_2),(\pi_2^*,\hat{\theta}_1))$
 are a \textbf{\textit{learnable  equilibria}} if 
\begin{equation}
  \pi_i^* \in \arg\max_{\pi_i} \bar{u}_i(\pi_i, \phi_{-i}^{\hat{\theta}^*_{-i}}(\pi_i),\theta_i), ~\forall i.
\end{equation}
and $\hat{\theta}_i$ are measurable w.r.t. the data available to each player, and this data comes from players playing some strategies $(\pi_i^{**},\pi_{-i}^{**})$m which may be a Nash equilibrium, some other equilibrium, or not an eq. at all.


\subsubsection{Existence of Learnable Equilibria}
Assume there are only two players.
\begin{theorem}
There exists a Learnable equilibrium in mixed strategies.
\end{theorem}


\begin{proof}
Let $\pi_i: A_i \to \Delta_{A_i}$ denote mixed strategies over the probability simplex $\Delta_{A_i}$. Let $\phi_i: \Delta_{A_{-i}} \to \Delta_{A_i}$ be the best response model of player $i$ used by player $-i$. We will consider it parametrized by $\theta_i \in \Theta$, a compact set. Denote the graph of $\phi_i$ by 
$$\Phi_i^{\theta_i}:= \{(\pi_{-i}, \phi_i^{\theta_i}(\pi_{-i}) : \pi_{-i} \in \Delta_{A_{-i}}\}.$$
Let 
\[
\Psi_1(\Phi_2^{\theta_2}) = \arg \max_{\pi_1} \bar{u}_1(\pi_1,\phi_2^{\theta_2}(\pi_1)).
\]
This can be seen as a function $\Psi_1^*(\theta_2)$. Note that it is a correspondence (a set-valued function). Thus, $\Psi_1 : \Delta_{A_1} \times \Delta_{A_2} \to 2^{\Delta_{A_1}}$. Similarly for $\Psi_2$. Then, $\Psi = (\Psi_1,\Psi_2) : \Delta_{A_1} \times \Delta_{A_2} \to 2^{\Delta_{A_1} \times \Delta_{A_2}}$.  

Denote $\Sigma = \Delta_{A_1} \times \Delta_{A_2}$ is non-empty, compact and convex and subsets of a Euclidean space.

Next, we note the $\bar{u}_i(\pi_1,\pi_2) = \mathbb{E}_{\pi_1,\pi_2}[u_i(a_1,a_2)]$. The functions  $\bar{u}_i$ are thus continuous and convex in $(\pi_1,\pi_2)$. And so are $\Psi_i$. Thus, $\Psi$ is as well. It is also non-empty since $\pi_i \in \Delta_{A_i}$, which are compact sets. 

We next prove upper-hemicontinuity of $\Psi$. Let $f_1((\pi_1,\pi_2),\theta_2) := \bar{u}_1(\pi_1,\pi_{2})$, where $(\pi_1,\pi_{2}) \in \bar{\Psi}_1(\theta_2):=\{(\pi_1,\pi_2): \pi_2 \in \phi_2^{\theta_2}(\pi_1), \pi_1 \in \Delta_{A_1}\}.$ Note that $f_1$ is a continuous function of $((\pi_1,\pi_2),\theta_2)$. $\bar{\Psi}_1$ is compact-valued since $\Delta_{A_1}$ is compact and $\phi_2^{\theta_2}$ is a continuous function in $\pi_1$. $\bar{\Psi}_1$ is also a continuous function of $\theta_2$ since $\phi_2^{\theta_2}(.)$ can be seen as a  continuous function of $\theta_2$. Then, by Berge's Maximum Theorem, 
$$\Psi_1^*(\theta_2) : = \arg \max \{f_1((\pi_1,\pi_2),\theta_2): (\pi_1,\pi_2) \in \bar{\Psi}_1(\theta_2)\}$$
is upper-hemicontinuous and compact-valued. Similarly, we can argue for $\Psi_2^*$, and thus $\Psi^*=(\Psi_1^*,\Psi_2^*)$ is also upper-hemicontinuous and compact-valued.

Now, by Kakutani's Fixed Point Theorem, there exists a fixed point $(\theta_1^*,\theta_2^*)$ of $\Psi^*$. But that implies, there exists a fixed point $(\Phi_1^{\theta_2^*},\Phi_2^{\theta_1^*})$. Equivalently, there exists a pair $(\phi_1^{\theta_2^*},\phi_2^{\theta_1^*})$. 

[What have we proved?]


%Since the parametric form of $phi_i^{\theta}$ is fixed, we can also think of the above as a function of $\theta_2$, and denote it as $\tilde{\Psi_1}(\theta_2)$. We can similarly define $\tilde{\Psi_2}(\theta_1)$


 
\end{proof}




\subsection{\bf\sf Learning Algorithms}

Now consider the following repeated game setting. Suppose each player knows its own $\theta$, but does not know that of the other. Let $\hat{\theta}_{i}^{k}$ denote the estimate of $\theta_i$ at time $k$ by player $-i$. To ease notation, we will write $\phi_i^{\theta_i}(a)$ as $\phi_i(a ; \theta_i)$.

Then, player $i$'s decision problem at time $k$ is
\[
\tilde{a}_i^k = \arg \max_{a_i} u_i(a_i,\phi_{-i}(a_i, \hat{\theta}^k_{-i})), 
\]
i.e., player $i$ uses an estimate of player $-i$'s best response at time $k$. The above optimization problem could be easy or difficult to solve depending on form of payoff functions and of the behavioral best response functions. 

Let $\mathcal{I}_k$ denote the common information at time $k$, which is the sequence of action-tuples so far. Let us denote an estimation function by 
\[
\hat{\theta}_i^k = g_i^k(\mathcal{I}_k).
\]
Let $\Gamma_i^k := (\phi_{-i}(\cdot ; \cdot), g_i^k)$, a parametric model of other players' best response and an estimator of the  parameters. We will call this the \textit{learning algorithm} used by player $i$ at time $k$. Denote $\Gamma_i = (\Gamma_i^1, \Gamma_i^k, \cdots)$ and $\Gamma = (\Gamma_i, \Gamma_{-i})$. We will call $\Gamma$ the \textbf{\textit{learning algorithm}}.

\begin{mdframed}
\noindent\textbf{Question 1:} Under what conditions on payoff functions and parameter set $\Theta$ does a learnable equilibrium exist?
\end{mdframed}

\begin{mdframed}
\noindent\textbf{Question 2:} Under what conditions on $u$, $\theta$, and $\Gamma$ does $(\tilde{a}_i^k,\tilde{a}_{-i}^k)$ converge? Does it converge to a learnable equilibrium?
\end{mdframed}

\begin{mdframed}
\noindent\textbf{Question 3:} Under what conditions does the learnable equilibrium coincide with a classical solution concept?
\end{mdframed}

Problems with the above: (1) Best response of a learning agent is changing as it learns the parameters of the best response of the other player. May not converge. But perhaps the operator is a contraction, so it just might work. 

\section{\bf\sf Sequential Games}

\subsection{\bf\sf Models of Behavior}

We now consider a Markov game as an instance of a sequential game. Denote the Q-value function,
\[
Q_i^{\pi_1,\pi_2}(s, a_1,a_2) = \mathbb{E}[\sum_{t=0}^{\infty}\gamma^t r_i(s_t,\pi_1(s_t),\pi_2(s_t)) | a^0 = (a_1,a_2)].
\]
We say that $(\pi_1^*,\pi_2^*)$ is a \textit{Markov (perfect?) equilibrium} if 
\[
Q_i^{\pi_i^*,\pi_{-i}^*}(s, a_1,a_2) \geq Q_i^{\pi_i,\pi_{-i}^*}(s, a_1,a_2),~~\forall \pi_i,~~\forall s, (a_1,a_2),~~\forall i.
\]
($a_i = \pi_i^*(s)?$). Denote $Q_i^{*,*}=Q_i^{\pi_i^*,\pi_{-i}^*}$ and 
\[
V_i^*(s) = Q_i^{*,*}(s, \pi_1^*(s),\pi_2^*(s)).
\]
Then, the equilibrium policy for player can be inferred as 
\[
\pi^*_1 (s) = \arg \max_{a_1} Q_i^{*,*}(s, a_1,\pi_2^*(s)).
\]


Now let us define best response of player $i$ to player $-i$ using a policy $\pi_{-i}$,
\begin{eqnarray}
\phi_i(\pi_{-i}(\cdot), s) &=& \arg\max_{a_i} Q_i^{*,\pi_{-i}}(s,a_i,\pi_{-i}(s)), ~\text{where}~Q_i^{*,\pi_{-i}}~\text{satisfies}\nonumber\\
\label{eq:exactFP}Q_i^{*,\pi_{-i}}(s,a_i,\pi_{-i}(s)) &=& r_i(s,a_i,\pi_{-i}(s)) + \mathbb{E}[\max_b Q_i^{*,\pi_{-i}}(s',b,\pi_{-i}(s))|s,a_i].
\end{eqnarray}
Now, the \textit{MPE} can be defined in terms of these best responses,
\[
\pi_i^*(s) = \phi_i(\pi_{-i}^*,s),~\text{and}~
\pi_{-i}^*(s) = \phi_{-i}(\pi_{i}^*,s),~~\forall s.
\]

Now, let us parametrize the best response $\phi_i$ by $\theta_i$, i.e., $\phi_i \approx \phi_i^{\theta_i}, \theta_i \in \Theta$. As before, we will call these \textit{behavioral best responses}. These parametric functions could even be `non-parametric' models such as neural networks, where the parameters are its weights. We will simplify notation to denote $Q_i^{*,\phi_{-i}^{\theta_{-i}}}$ as $Q_i^{*,\theta_{-i}}$, etc. Further, let us denote a constant policy that plays action $a$ (in all states) as $\bf 1_a$. Then, given this ``behavioral model" for the other player, each player's decision problem becomes (check!)
\begin{eqnarray}
\tilde{\pi}_i(s) &=& \arg\max_{a_i} Q_i^{*,\theta_{-i}}(s,a_i,\phi_{-i}^{\theta_{-i}}({\bf 1_{a_i}},s)), ~\text{where}~Q_i^{*,\theta_{-i}}~\text{satisfies}\nonumber\\
\label{eq:approxFP}Q_i^{*,\theta_{-i}}(s,a_i,\phi_{-i}^{\theta_{-i}}({\bf 1_{a_i}},s)) &=& r_i(s,a_i,\phi_{-i}^{\theta_{-i}}({\bf 1_{a_i}},s)) + \mathbb{E}[\max_b Q_i^{*,\theta_{-i}}(s',b,\phi_{-i}^{\theta_{-i}}({\bf 1_{b}},s))|s,a_i].
\end{eqnarray}
The parameters $\theta = (\theta_i, \theta_{-i})$ models the best response of the other player. 

\subsection{\bf\sf Learnable Solution Concepts}

We say that  $(\tilde{\pi}_i^*,\tilde{\pi}_{-i}^*)$ is a \textbf{\textit{learnable sequential equilibrium}} if there exist $(\theta_i, \theta_{-i}) \in \Theta \times \Theta$ such that 
\[
\tilde{\pi}_i^*(s) = \phi_i^{\theta_i}(\tilde{\pi}_{-i}^*,s),~\text{and}~
\tilde{\pi}_{-i}^*(s) = \phi_{-i}^{\theta_{-i}}(\tilde{\pi}_{i}^*,s),~~\forall s.
\]
i.e., if there exists a parametrization of the best response functions such that a fixed point exists in the parametric best responses, then it is called a learnable sequential equilibria.

\subsection{\bf\sf Learning Algorithms}

Let $\hat{\theta}_{i}^{k}$ denote the estimate of $\theta_i$ at time $k$ by player $-i$. To ease notation, we will write $\phi_i^{\theta_i}(\pi,s)$ as $\phi_i(\pi, s; \theta_i)$. Then, player $i$'s decision problem at time $k$ is (check!)
\[
\tilde{\pi}_i^k(s) = \arg\max_{a_i} Q_i^{*,\theta_{-i}}(s,a_i,\phi_{-i}^{\theta_{-i}}({\bf 1_{a_i}},s)), ~\text{where}~Q_i^{*,\theta_{-i}}~\text{satisfies} ~\eqref{eq:exactFP}, 
\]
i.e., player $i$ uses an estimate of player $-i$'s best response at time $k$. The above optimization problem could be easy or difficult to solve depending on form of payoff functions and of the behavioral best response functions. 

Let $\mathcal{I}_k$ denote the common information at time $k$, which is the sequence of action-tuples so far. Let us denote an estimation function by 
\[
\hat{\theta}_i^k = g_i^k(\mathcal{I}_k).
\]
Let $\Gamma_i^k := (\phi_{-i}(\cdot ; \cdot), g_i^k)$, a parametric model of other players' best response and an estimator of the  parameters. We will call this the \textit{learning algorithm} used by player $i$ at time $k$. Denote $\Gamma_i = (\Gamma_i^1, \Gamma_i^k, \cdots)$ and $\Gamma = (\Gamma_i, \Gamma_{-i})$. We will call $\Gamma$ the \textbf{\textit{learning algorithm}}.

\begin{mdframed}
\noindent\textbf{Question 1:} Under what conditions on payoff functions and parameter set $\Theta$ does a learnable sequential equilibrium exist?
\end{mdframed}

\begin{mdframed}
\noindent\textbf{Question 2:} Under what conditions on $r$, transition model $\delta$, $\theta$, and $\Gamma$ does $(\tilde{\pi}_i^k,\tilde{\pi}_{-i}^k)$ converge? Does it converge to a learnable sequential equilibrium?
\end{mdframed}

\begin{mdframed}
\noindent\textbf{Question 3:} Under what conditions does the learnable sequential equilibrium coincide with a classical solution concept?
\end{mdframed}

\section{\bf\sf Incomplete Information (PLACEHOLDER)}

\subsection{\bf\sf Models of Behavior}

We will consider a Markov game with partial observations as a model of a sequential game with incomplete information. Let $H_k$ define the history of states and actions by time $k$. Let $I_k$ and $h_k^i$ denote the common and private information available player $i$ at time $k$. Denote $I_k^i = I_k + h_k^i$. We will abuse notation for $I_k^i$ to also mean its information statistic, i.e., the belief (conditional probability distribution) over the state given the information in $I_k^i$. Note that strategies $\pi_i(I_k^i)$, i.e., map from the information state to the probability simplex over actions.

Now, we can denote the Q-value function as
\[
Q_{i,k}^{\pi_1,\pi_2}(I_k^i, a_1,a_2) := \mathbb{E}[\sum_{t=k}^{\infty}\gamma^t r_i(s_t,\pi_1(I_t^1),\pi_2(I_t^2)) | I_k^1, a^0 = (a_1,a_2)].
\]
We say that $(\pi_1^*,\pi_2^*)$ is a \textit{Markov (perfect?) equilibrium} if 
\[
Q_{i,k}^{\pi_i^*,\pi_{-i}^*}(I_k^i, a_1, a_2) \geq Q_{i,k}^{\pi_i,\pi_{-i}^*}(I_k^i, a_1,a_2),~~\forall \pi_i,~~\forall I_k^i,   (a_1,a_2),~~\forall i.
\]
($a_i = \pi_i^*(s)?$). Denote $Q_{i,k}^{*,*}=Q_{i,k}^{\pi_i^*,\pi_{-i}^*}$. 
%\[ V_{i,k}^*(I_k^i) = Q_{i,k}^{*,*}(I_k^i,  \pi_1^*(I_k^1),\pi_2^*(I_k^2)). \]
Then, the equilibrium policy for player $i$ can be inferred as 
\[
\pi^*_i (I_k^i) = \arg \max_{a_i} Q_{i,k}^{*,*}(I_k^i, a_i,\pi_{-i}^*(I_k^{-i})).
\]
(NOT CORRECT)


Now let us define best response of player $i$ to player $-i$ using a policy $\pi_{-i}$,
\begin{eqnarray}
\phi_i(\pi_{-i}(\cdot), s) &=& \arg\max_{a_i} Q_{i,k}^{*,\pi_{-i}}(s,a_i,\pi_{-i}(s)), ~\text{where}~Q_{i,k}^{*,\pi_{-i}}~\text{satisfies}\nonumber\\
\label{eq:exactFP}Q_{i,k}^{*,\pi_{-i}}(s,a_i,\pi_{-i}(s)) &=& r_i(s,a_i,\pi_{-i}(s)) + \mathbb{E}[\max_b Q_{i,k}^{*,\pi_{-i}}(s',b,\pi_{-i}(s))|s,a_i].
\end{eqnarray}
Now, the \textit{MPE} can be defined in terms of these best responses,
\[
\pi_i^*(s) = \phi_i(\pi_{-i}^*,s),~\text{and}~
\pi_{-i}^*(s) = \phi_{-i}(\pi_{i}^*,s),~~\forall s.
\]

Now, let us parametrize the best response $\phi_i$ by $\theta_i$, i.e., $\phi_i \approx \phi_i^{\theta_i}, \theta_i \in \Theta$. As before, we will call these \textit{behavioral best responses}. These parametric functions could even be `non-parametric' models such as neural networks, where the parameters are its weights. We will simplify notation to denote $Q_{i,k}^{*,\phi_{-i}^{\theta_{-i}}}$ as $Q_{i,k}^{*,\theta_{-i}}$, etc. Further, let us denote a constant policy that plays action $a$ (in all states) as $\bf 1_a$. Then, given this ``behavioral model" for the other player, each player's decision problem becomes (check!)
\begin{eqnarray}
\tilde{\pi}_i(s) &=& \arg\max_{a_i} Q_{i,k}^{*,\theta_{-i}}(s,a_i,\phi_{-i}^{\theta_{-i}}({\bf 1_{a_i}},s)), ~\text{where}~Q_{i,k}^{*,\theta_{-i}}~\text{satisfies}\nonumber\\
\label{eq:approxFP}Q_{i,k}^{*,\theta_{-i}}(s,a_i,\phi_{-i}^{\theta_{-i}}({\bf 1_{a_i}},s)) &=& r_i(s,a_i,\phi_{-i}^{\theta_{-i}}({\bf 1_{a_i}},s)) + \mathbb{E}[\max_b Q_{i,k}^{*,\theta_{-i}}(s',b,\phi_{-i}^{\theta_{-i}}({\bf 1_{b}},s))|s,a_i].
\end{eqnarray}
The parameters $\theta = (\theta_i, \theta_{-i})$ models the best response of the other player. 

\subsection{\bf\sf Learnable Solution Concepts}

We say that  $(\tilde{\pi}_i^*,\tilde{\pi}_{-i}^*)$ is a \textbf{\textit{learnable sequential equilibrium}} if there exist $(\theta_i, \theta_{-i}) \in \Theta \times \Theta$ such that 
\[
\tilde{\pi}_i^*(s) = \phi_i^{\theta_i}(\tilde{\pi}_{-i}^*,s),~\text{and}~
\tilde{\pi}_{-i}^*(s) = \phi_{-i}^{\theta_{-i}}(\tilde{\pi}_{i}^*,s),~~\forall s.
\]
i.e., if there exists a parametrization of the best response functions such that a fixed point exists in the parametric best responses, then it is called a learnable sequential equilibria.

\subsection{\bf\sf Learning Algorithms}

Let $\hat{\theta}_{i}^{k}$ denote the estimate of $\theta_i$ at time $k$ by player $-i$. To ease notation, we will write $\phi_i^{\theta_i}(\pi,s)$ as $\phi_i(\pi, s; \theta_i)$. Then, player $i$'s decision problem at time $k$ is (check!)
\[
\tilde{\pi}_i^k(s) = \arg\max_{a_i} Q_{i,k}^{*,\theta_{-i}}(s,a_i,\phi_{-i}^{\theta_{-i}}({\bf 1_{a_i}},s)), ~\text{where}~Q_{i,k}^{*,\theta_{-i}}~\text{satisfies} ~\eqref{eq:exactFP}, 
\]
i.e., player $i$ uses an estimate of player $-i$'s best response at time $k$. The above optimization problem could be easy or difficult to solve depending on form of payoff functions and of the behavioral best response functions. 

Let $\mathcal{I}_k$ denote the common information at time $k$, which is the sequence of action-tuples so far. Let us denote an estimation function by 
\[
\hat{\theta}_i^k = g_i^k(\mathcal{I}_k).
\]
Let $\Gamma_i^k := (\phi_{-i}(\cdot ; \cdot), g_i^k)$, a parametric model of other players' best response and an estimator of the  parameters. We will call this the \textit{learning algorithm} used by player $i$ at time $k$. Denote $\Gamma_i = (\Gamma_i^1, \Gamma_i^k, \cdots)$ and $\Gamma = (\Gamma_i, \Gamma_{-i})$. We will call $\Gamma$ the \textbf{\textit{learning algorithm}}.

\begin{mdframed}
\noindent\textbf{Question 1:} Under what conditions on payoff functions and parameter set $\Theta$ does a learnable sequential equilibrium exist?
\end{mdframed}

\begin{mdframed}
\noindent\textbf{Question 2:} Under what conditions on $r$, transition model $\delta$, $\theta$, and $\Gamma$ does $(\tilde{\pi}_i^k,\tilde{\pi}_{-i}^k)$ converge? Does it converge to a learnable sequential equilibrium?
\end{mdframed}

\begin{mdframed}
\noindent\textbf{Question 3:} Under what conditions does the learnable sequential equilibrium coincide with a classical solution concept?
\end{mdframed}

%\section{\bf\sf Bayesian Games}

\end{document}
