# Supplementary material for: Correlated Quantal Response Equilibrium: A New Equilibrium Notion for Human-AI Strategic Interactions
Source: arXiv:2610.29020 source file (2026-10-21)
Supplement: Supplementary file 4 [file main.tex]

\documentclass[11pt]{article}
\usepackage{subcaption}
\usepackage{graphicx}
\graphicspath{{plots/}}
\captionsetup[subfigure]{justification=centering}

% --- Core math & symbols ---
\usepackage{amsmath, amssymb, amsfonts, mathtools}
\usepackage{bm}
\usepackage{amsthm}
\newtheorem{theorem}{Theorem}
\newtheorem{definition}{Definition}
\newtheorem{proposition}{Proposition}

% --- Tables & figures ---
\usepackage{graphicx}
\usepackage{booktabs}
\usepackage{array}
\usepackage{caption}
\captionsetup{font=small}

% --- Typography & layout ---
\usepackage[margin=1in]{geometry}
\usepackage{microtype}
\usepackage{lmodern}
\usepackage{xcolor}
\usepackage{enumitem}

% --- Hyperlinks & references ---
\usepackage[hidelinks]{hyperref}
\usepackage[nameinlink]{cleveref}

% --- Handy macros ---
\newcommand{\Unif}{\mathrm{Unif}}
\newcommand{\QBR}{\mathrm{QBR}}
\newcommand{\E}{\mathbb{E}}
\newcommand{\R}{\mathbb{R}}
\newcommand{\Aone}{\mathcal{A}_1}
\newcommand{\Atwo}{\mathcal{A}_2}
\newcommand{\KL}{D_{\mathrm{KL}}}
\newcommand{\Hist}{\rho_{\mathrm{hist}}}
\newcommand{\Future}{\rho_{\mathrm{future}}}
\newcommand{\Marg}{\rho_{\mathrm{marg}}}
\newcommand{\QR}{\rho_{\mathrm{QR}}}
\newcommand{\Theory}{\rho^{\star}_{\epsilon_{\mathrm{relax}}}}

\title{\texttt{learn\_eq}}
\author{Andy}
\date{October 2025}

\begin{document}
\maketitle

\paragraph{Problem formulation.}
We consider a finite two-player normal-form game with action sets $A_1,A_2$ and utilities $U_1,U_2$.
A joint distribution $\rho\in\Delta(A_1\times A_2)$ specifies how often each action pair $(a_1,a_2)$ is played.
For player 1, fixing a recommended action $a_1$, define the reweighted utility
\[
\tilde U_{1,a_1}(\tilde a_1,a_2)=\rho(a_1,a_2)U_1(\tilde a_1,a_2).
\]
Then the correlated-equilibrium obedience condition can be written as: for every $a_1\in A_1$,
\[
\delta_{a_1}
\in
\arg\max_{\pi_1\in\Delta(A_1)}
\sum_{\tilde a_1,a_2}
\pi_1(\tilde a_1)\tilde U_{1,a_1}(\tilde a_1,a_2).
\]
This avoids the usual conditioning issue when $\rho(a_1)=0$.

To obtain a quantal or relaxed version, we keep the same obedience structure but allow a nonnegative slack.
The optimization problem is
\begin{align*}
    \min_{\rho(\cdot,\cdot)\in\Delta(A_1\otimes A_2)}
    &\sum_{(a_1,a_2)\in A_1\otimes A_2}\rho(a_1,a_2)\log\rho(a_1,a_2) \\
    \text{subject to } \\
    \forall a_1\in A_1\qquad
    \sum_{a_2\in A_2}\rho(a_1,a_2)U_1(a_1,a_2)
    &\ge
    \max_{\pi_1\in\Delta(A_1)}
    \sum_{\tilde a_1,a_2}
    \pi_1(\tilde a_1)\rho(a_1,a_2)U_1(\tilde a_1,a_2)-\gamma_{a_1}, \\
    \forall a_2\in A_2\qquad
    \sum_{a_1\in A_1}\rho(a_1,a_2)U_2(a_1,a_2)
    &\ge
    \max_{\pi_2\in\Delta(A_2)}
    \sum_{a_1,\tilde a_2}
    \pi_2(\tilde a_2)\rho(a_1,a_2)U_2(a_1,\tilde a_2)-\gamma_{a_2}.
\end{align*}
If $\gamma=0$, the feasible set is exactly the set of correlated equilibria, so the objective selects the maximum-entropy CE.
In the experiments below, following the discussion in the meeting, we use one common scalar slack and write $\gamma_{a_i}\equiv\epsilon_{\mathrm{relax}}$.

The constraints can be rewritten in the familiar linear form.
For player 1, for example,
\begin{align*}
    \sum_{a_2\in A_2}\rho(a_1,a_2)U_1(a_1,a_2)
    &\ge
    \sum_{a_2\in A_2}\rho(a_1,a_2)U_1(\tilde a_1,a_2)-\gamma_{a_1},
    \qquad \forall \tilde a_1\in A_1\setminus\{a_1\}.
\end{align*}
Thus the problem is a convex program over the simplex with linear obedience constraints.
Introducing Lagrange multipliers $\lambda_{a_i,\tilde a_i}\ge 0$, one obtains the equivalent exponential-family form
\begin{align*}
    \rho(a_1,a_2)
    \propto
    \exp\Bigg(
    &\sum_{\tilde a_1\in A_1\setminus\{a_1\}}
    \lambda_{a_1,\tilde a_1}\big(U_1(a_1,a_2)-U_1(\tilde a_1,a_2)\big) \\
    +
    &\sum_{\tilde a_2\in A_2\setminus\{a_2\}}
    \lambda_{a_2,\tilde a_2}\big(U_2(a_1,a_2)-U_2(a_1,\tilde a_2)\big)
    \Bigg).
\end{align*}
Hence the correlated QRE family is parameterized by the nonnegative multipliers
$\{\lambda_{a_i,\tilde a_i}\}_{i\in\{1,2\},a_i\in A_i,\tilde a_i\in A_i\setminus\{a_i\}}$.

\begin{theorem}[Existence]
Let $A_1$ and $A_2$ be finite action sets, let $U_1,U_2$ be bounded utility functions, and let $\gamma\ge 0$.
Consider the optimization problem
\[
\min_{\rho\in\Delta(A_1\times A_2)}
\sum_{(a_1,a_2)\in A_1\times A_2}\rho(a_1,a_2)\log\rho(a_1,a_2)
\]
subject to the obedience constraints
\[
\sum_{a_2}\rho(a_1,a_2)\big(U_1(\tilde a_1,a_2)-U_1(a_1,a_2)\big)
\le \gamma_{a_1},
\qquad \forall a_1\in A_1,\ \forall \tilde a_1\neq a_1,
\]
and
\[
\sum_{a_1}\rho(a_1,a_2)\big(U_2(a_1,\tilde a_2)-U_2(a_1,a_2)\big)
\le \gamma_{a_2},
\qquad \forall a_2\in A_2,\ \forall \tilde a_2\neq a_2.
\]
Then this problem admits at least one minimizer.
\end{theorem}

\begin{proof}
Let $K_\gamma$ denote the feasible set.
Because the game is finite, there exists a mixed Nash equilibrium $(\sigma_1,\sigma_2)$.
The associated product distribution $\bar\rho(a_1,a_2)=\sigma_1(a_1)\sigma_2(a_2)$ satisfies all obedience constraints with slack at most $0$, hence $\bar\rho\in K_\gamma$ whenever $\gamma\ge 0$.
Therefore $K_\gamma$ is nonempty.
Moreover, $K_\gamma$ is a closed subset of the simplex $\Delta(A_1\times A_2)$, which is compact in finite dimensions, so $K_\gamma$ is compact.
Finally, with the convention $0\log 0:=0$, the objective is continuous on $K_\gamma$.
By the Weierstrass theorem, it attains its minimum.
\end{proof}

\begin{theorem}[Uniqueness]
Under the same assumptions, the optimization problem admits a unique minimizer.
\end{theorem}

\begin{proof}
The feasible set $K_\gamma$ is convex because it is the intersection of the simplex with linear constraints.
The function $x\mapsto x\log x$ is strictly convex on $[0,1]$, so
\[
F(\rho)=\sum_{(a_1,a_2)\in A_1\times A_2}\rho(a_1,a_2)\log\rho(a_1,a_2)
\]
is strictly convex on $\Delta(A_1\times A_2)$ and hence on $K_\gamma$.
A strictly convex function has at most one minimizer on a convex set.
\end{proof}

\clearpage

\section{Experiment Design}


The experiment is predictive.
For each game, we observe the first $T$ rounds of a trajectory, build several candidate predictors of joint play from that history, and ask which predictor is closest to the next $H$ rounds.
The target of prediction is therefore a future empirical joint distribution


For each game and each history length $T$, the procedure is:
\begin{enumerate}[leftmargin=2.2em,itemsep=0.2em,topsep=0.2em]
    \item generate one long trajectory of play,
    \item use rounds $1{:}T$ as history,
    \item build four candidate predictors from the history,
    \item use rounds $T{+}1{:}T{+}H$ as held-out future,
    \item score each predictor against that future block.
\end{enumerate}
This makes the evaluation genuinely out-of-sample.

\paragraph{history--future split.}
We study finite two-player normal-form games with action sets $A_1$ and $A_2$ and utilities $U_1,U_2$.
For each game and random seed, we generate one trajectory
\[
\{(a_{1,t},a_{2,t})\}_{t=1}^{T_{\max}+H}
\]
of joint play, where $T_{\max}$ is the largest history length and $H$ is a fixed holdout window.
For each prefix length $T\in\{100,300,1000,3000,10000\}$, we define the history empirical joint distribution
\begin{equation}
\Hist^{(T)}(a_1,a_2)
=
\frac{1}{T}\sum_{t=1}^{T}\mathbf 1\{(a_{1,t},a_{2,t})=(a_1,a_2)\},
\label{eq:hist-joint}
\end{equation}
and the future empirical joint distribution over the next $H$ plays,
\begin{equation}
\Future^{(T,H)}(a_1,a_2)
=
\frac{1}{H}\sum_{t=T+1}^{T+H}\mathbf 1\{(a_{1,t},a_{2,t})=(a_1,a_2)\}.
\label{eq:future-joint}
\end{equation}
Equation~\eqref{eq:hist-joint} is the training object and \eqref{eq:future-joint} is the testing object.
The main question is: among the candidate predictors built from the history, which one minimizes
$\KL(\Future^{(T,H)}\|Q)$?

\paragraph{Offline data generation: smoothed fictitious play.}
We generate trajectories using a stochastic smoothed fictitious-play process.
At time $t$, the simulator stores exponentially smoothed beliefs
$FP_{1,t}\in\Delta(A_1)$ and $FP_{2,t}\in\Delta(A_2)$, initialized uniformly.
Each player first samples a proxy action from its belief about the opponent,
\begin{align}
    a_2' &\sim FP_{2,t}, & a_1' &\sim FP_{1,t},
\end{align}
and then responds to that proxy action using a soft best response:
\begin{align}
    a_{1,t} &\sim \mathrm{SoftBR}_1(\cdot\mid a_2'), \\
    a_{2,t} &\sim \mathrm{SoftBR}_2(\cdot\mid a_1').
\end{align}
The soft best-response distributions are
\begin{align}
\mathrm{SoftBR}_1(a_1\mid a_2')
&=
\frac{\exp(U_1(a_1,a_2')/\tau_1)}{\sum_{\tilde a_1\in A_1}\exp(U_1(\tilde a_1,a_2')/\tau_1)},
\\
\mathrm{SoftBR}_2(a_2\mid a_1')
&=
\frac{\exp(U_2(a_1',a_2)/\tau_2)}{\sum_{\tilde a_2\in A_2}\exp(U_2(a_1',\tilde a_2)/\tau_2)}.
\end{align}
Beliefs are then updated by exponential moving average,
\begin{align}
FP_{1,t+1} &= \alpha FP_{1,t} + (1-\alpha)\mathbf e_{a_{1,t}},\\
FP_{2,t+1} &= \alpha FP_{2,t} + (1-\alpha)\mathbf e_{a_{2,t}}.
\end{align}
In the current implementation, we keep all generated samples and do \emph{not} discard burn-in.

\paragraph{ one-step joint factorizes}
Conditional on $(FP_{1,t},FP_{2,t})$, the one-step joint distribution is
\begin{align}
P_t(a_1,a_2)
&:=
\Pr(a_{1,t}=a_1,a_{2,t}=a_2\mid FP_{1,t},FP_{2,t}) \\
&=
\sum_{a_1',a_2'}
\Pr(a_1'\mid FP_{1,t})\Pr(a_2'\mid FP_{2,t})
\Pr(a_{1,t}=a_1\mid a_2')
\Pr(a_{2,t}=a_2\mid a_1') \\
&=
\Bigg(\sum_{a_2'\in A_2}FP_{2,t}(a_2')\,\mathrm{SoftBR}_1(a_1\mid a_2')\Bigg)
\Bigg(\sum_{a_1'\in A_1}FP_{1,t}(a_1')\,\mathrm{SoftBR}_2(a_2\mid a_1')\Bigg).
\label{eq:pt-factorization}
\end{align}
So each instantaneous joint distribution is product-form.
The empirical history joint $\Hist^{(T)}$ averages these product-form distributions over time, so it need not be exactly product, but under this simulator we should not expect strong within-round correlation.

\paragraph{Predictor 1: direct history joint.}
The first predictor is simply the history empirical joint itself:
\[
Q=\Hist^{(T)}.
\]
This is the most direct baseline: predict that the next $H$ rounds will look like the first $T$ rounds.

\paragraph{Predictor 2: product of empirical marginals.}
From the history prefix, define marginal counts
\[
N_1(a_1)=\#\{t\le T: a_{1,t}=a_1\},
\qquad
N_2(a_2)=\#\{t\le T: a_{2,t}=a_2\}.
\]
We smooth these counts with a small pseudo-count $\epsilon_{\mathrm{smooth}}>0$:
\begin{align}
q_1^{(T)}(a_1)
&=
\frac{N_1(a_1)+\epsilon_{\mathrm{smooth}}}{T+|A_1|\epsilon_{\mathrm{smooth}}},
\\
q_2^{(T)}(a_2)
&=
\frac{N_2(a_2)+\epsilon_{\mathrm{smooth}}}{T+|A_2|\epsilon_{\mathrm{smooth}}}.
\label{eq:smooth-marginals}
\end{align}
The denominator includes $|A_i|\epsilon_{\mathrm{smooth}}$ because the pseudo-count is added once to each of the $|A_i|$ actions, so the total mass must also increase by that amount.
The second predictor is the product joint
\begin{equation}
\Marg^{(T)}(a_1,a_2)=q_1^{(T)}(a_1)q_2^{(T)}(a_2).
\label{eq:marg-product}
\end{equation}
This predictor keeps only marginal action frequencies and discards all joint dependence.

\paragraph{Predictor 3: unconditional quantal-response product.}
Using the same smoothed marginals, define unconditional expected utilities
\begin{align}
u_1^{(T)}(a_1)
&=
\sum_{a_2\in A_2}q_2^{(T)}(a_2)U_1(a_1,a_2),
\\
u_2^{(T)}(a_2)
&=
\sum_{a_1\in A_1}q_1^{(T)}(a_1)U_2(a_1,a_2).
\end{align}
Then define unconditional quantal-response policies
\begin{align}
\pi_1^{(T)}(a_1)
&=
\frac{\exp(\beta u_1^{(T)}(a_1))}{\sum_{\tilde a_1\in A_1}\exp(\beta u_1^{(T)}(\tilde a_1))},
\\
\pi_2^{(T)}(a_2)
&=
\frac{\exp(\beta u_2^{(T)}(a_2))}{\sum_{\tilde a_2\in A_2}\exp(\beta u_2^{(T)}(\tilde a_2))}.
\end{align}
The corresponding joint predictor is the exact outer product
\begin{equation}
\QR^{(T)}(a_1,a_2)=\pi_1^{(T)}(a_1)\pi_2^{(T)}(a_2).
\label{eq:qr-product}
\end{equation}
In matrix notation, this is $\QR^{(T)}=\pi_1^{(T)}(\pi_2^{(T)})^\top$.
So the third predictor is still independent across players, but its marginals are not raw frequencies; they are quantal responses induced from those frequencies.

\paragraph{Predictor 4: maximum-entropy relaxed obedience.}
For a common scalar relaxation level $\epsilon_{\mathrm{relax}}\ge 0$, define
\begin{align}
\mathcal K_{\epsilon_{\mathrm{relax}}}
:=
\Big\{\rho\in\Delta(A_1\times A_2):
&\sum_{a_2}\rho(a_1,a_2)\big(U_1(\tilde a_1,a_2)-U_1(a_1,a_2)\big)
\le \epsilon_{\mathrm{relax}}, \\
&\hspace{5em}\forall a_1\in A_1,\ \forall \tilde a_1\neq a_1, \\
&\sum_{a_1}\rho(a_1,a_2)\big(U_2(a_1,\tilde a_2)-U_2(a_1,a_2)\big)
\le \epsilon_{\mathrm{relax}}, \\
&\hspace{5em}\forall a_2\in A_2,\ \forall \tilde a_2\neq a_2
\Big\}.
\end{align}
The fourth predictor is the maximum-entropy point in this feasible set,
\begin{equation}
\Theory
=
\arg\min_{\rho\in\mathcal K_{\epsilon_{\mathrm{relax}}}}
\sum_{(a_1,a_2)}\rho(a_1,a_2)\log\rho(a_1,a_2).
\label{eq:theory-predictor}
\end{equation}
The main setting is $\epsilon_{\mathrm{relax}}=0$, with additional fixed values $\{0.01,0.05,0.10\}$ used as sensitivity checks.
Unlike the first three predictors, this predictor is defined directly from the game payoffs and the relaxation level.

\paragraph{Primary held-out metric.}
For any candidate predictor $Q\in\Delta(A_1\times A_2)$, the main score is held-out KL divergence,
\begin{equation}
\mathrm{KL}_{\mathrm{pred}}(Q;T,H)
=
\KL\!\left(\Future^{(T,H)}\,\middle\|\,Q\right)
=
\sum_{a_1,a_2}\Future^{(T,H)}(a_1,a_2)
\log\frac{\Future^{(T,H)}(a_1,a_2)}{Q(a_1,a_2)}.
\label{eq:heldout-kl}
\end{equation}

\eqref{eq:heldout-kl}  asks how close the model distribution $Q$ is to the actual empirical distribution of the next $H$ rounds.

We evaluate the candidate set
\[
Q\in\Big\{\Hist^{(T)},\ \Marg^{(T)},\ \QR^{(T)},\ \rho_{\epsilon_{\mathrm{relax}}}^{\star}\Big\}.
\]
So, operationally, the experiment asks which of the four predictors is closest to the held-out future joint.

% We also report the average future log-likelihood
% \begin{equation}
% \mathcal L_{\mathrm{pred}}(Q;T,H)
% =
% \frac{1}{H}\sum_{t=T+1}^{T+H}\log Q(a_{1,t},a_{2,t})
% =
% \sum_{a_1,a_2}\Future^{(T,H)}(a_1,a_2)\log Q(a_1,a_2).
% \label{eq:heldout-ll}
% \end{equation}
% The two metrics are exactly related by
% \begin{equation}
% \KL\!\left(\Future^{(T,H)}\,\middle\|\,Q\right)
% =
% -\mathcal H\!\left(\Future^{(T,H)}\right)-\mathcal L_{\mathrm{pred}}(Q;T,H),
% \label{eq:kl-ll-identity}
% \end{equation}
% where $\mathcal H(P):=-\sum_x P(x)\log P(x)$ is Shannon entropy.
% Because the entropy term depends only on the future data and not on $Q$, minimizing held-out KL is exactly equivalent to maximizing held-out average log-likelihood.

\paragraph{in sample distance}
The held-out metric in \eqref{eq:heldout-kl} is the main evaluation.
In addition, we use proxy diagnostics to understand \emph{why} a predictor does or does not work.
The generic proxy score is
\begin{equation}
\mathrm{KL}_{\mathrm{proxy}}(Q;T)
=
\KL\!\left(\Hist^{(T)}\,\middle\|\,Q\right).
\label{eq:proxy-kl}
\end{equation}
In particular, we report
\[
\KL(\Hist^{(T)}\|\Marg^{(T)}),
\qquad
\KL(\Hist^{(T)}\|\QR^{(T)}),
\qquad
\KL(\Hist^{(T)}\|\rho_{\epsilon_{\mathrm{relax}}}^{\star}).
\]
These diagnostics have different meanings:
\begin{itemize}[leftmargin=1.8em,itemsep=0.2em,topsep=0.2em]
    \item $\KL(\Hist\|\Marg)$ measures how much joint structure is lost when we collapse the history to marginal frequencies and impose independence.
    \item $\KL(\Hist\|\QR)$ measures the additional distortion introduced by replacing raw marginals with quantal-response marginals.
    \item $\KL(\Hist\|\Theory)$ measures whether the theory predictor is already close to the observed history.
\end{itemize}


\paragraph{Theory sensitivity with respect to $\epsilon_{\mathrm{relax}}$.}
Because the theory predictor depends on $\epsilon_{\mathrm{relax}}$, we also study the maps
\begin{equation}
\begin{split}
\epsilon_{\mathrm{relax}} &\mapsto \KL\!\left(\Future^{(T,H)}\,\middle\|\,\rho^{\star}_{\epsilon_{\mathrm{relax}}}\right)
\end{split}
\label{eq:theory-heldout-sensitivity}
\end{equation}
Equation~\eqref{eq:theory-heldout-sensitivity} is the main sensitivity analysis because it answers the predictive question: which relaxation level gives the best held-out theory predictor?


\newpage

% =========================================================
% Main plots: held-out prediction
% =========================================================
\begin{figure}[t]
    \centering

    \begin{subfigure}[t]{0.48\textwidth}
        \centering
        \includegraphics[width=\linewidth]{matching_pennies_prediction.png}
        \caption{Matching Pennies}
    \end{subfigure}\hfill
    \begin{subfigure}[t]{0.48\textwidth}
        \centering
        \includegraphics[width=\linewidth]{rock_paper_scissors_prediction.png}
        \caption{Rock--Paper--Scissors}
    \end{subfigure}

    \vspace{0.6em}

    \begin{subfigure}[t]{0.48\textwidth}
        \centering
        \includegraphics[width=\linewidth]{prisoners_dilemma_prediction.png}
        \caption{Prisoner's Dilemma}
    \end{subfigure}\hfill
    \begin{subfigure}[t]{0.48\textwidth}
        \centering
        \includegraphics[width=\linewidth]{battle_of_the_sexes_prediction.png}
        \caption{Battle of the Sexes}
    \end{subfigure}

    \vspace{0.6em}

    \begin{subfigure}[t]{0.48\textwidth}
        \centering
        \includegraphics[width=\linewidth]{chicken_prediction.png}
        \caption{Chicken}
    \end{subfigure}\hfill
    \begin{subfigure}[t]{0.48\textwidth}
        \centering
        \includegraphics[width=\linewidth]{stag_hunt_prediction.png}
        \caption{Stag Hunt}
    \end{subfigure}

    \caption{
    Held-out prediction performance across six games.
    For each history size \(T\), the four candidate predictors
    \(\rho_{\mathrm{hist}}^{(T)}\),
    \(\rho_{\mathrm{marg}}^{(T)} = q_1^{(T)} \otimes q_2^{(T)}\),
    \(\rho_{\mathrm{QR}}^{(T)} = \pi_1^{(T)} \otimes \pi_2^{(T)}\),
    and \(\rho^\star_{\epsilon_{\mathrm{relax}}=0}\)
    are evaluated against the future empirical joint distribution
    \(\rho_{\mathrm{future}}^{(T,H)}\) using held-out KL divergence
    \(D_{\mathrm{KL}}(\rho_{\mathrm{future}}^{(T,H)} \,\|\, Q)\).
    Lower values are better.
    }
    \label{fig:prediction_all_games}
\end{figure}


% =========================================================
% Proxy diagnostics
% =========================================================
\begin{figure}[t]
    \centering

    \begin{subfigure}[t]{0.48\textwidth}
        \centering
        \includegraphics[width=\linewidth]{matching_pennies_proxy.png}
        \caption{Matching Pennies}
    \end{subfigure}\hfill
    \begin{subfigure}[t]{0.48\textwidth}
        \centering
        \includegraphics[width=\linewidth]{rock_paper_scissors_proxy.png}
        \caption{Rock--Paper--Scissors}
    \end{subfigure}

    \vspace{0.6em}

    \begin{subfigure}[t]{0.48\textwidth}
        \centering
        \includegraphics[width=\linewidth]{prisoners_dilemma_proxy.png}
        \caption{Prisoner's Dilemma}
    \end{subfigure}\hfill
    \begin{subfigure}[t]{0.48\textwidth}
        \centering
        \includegraphics[width=\linewidth]{battle_of_the_sexes_proxy.png}
        \caption{Battle of the Sexes}
    \end{subfigure}

    \vspace{0.6em}

    \begin{subfigure}[t]{0.48\textwidth}
        \centering
        \includegraphics[width=\linewidth]{chicken_proxy.png}
        \caption{Chicken}
    \end{subfigure}\hfill
    \begin{subfigure}[t]{0.48\textwidth}
        \centering
        \includegraphics[width=\linewidth]{stag_hunt_proxy.png}
        \caption{Stag Hunt}
    \end{subfigure}

    \caption{
    Proxy diagnostics across six games.
    These curves compare in-sample history-based objects, including
    \(D_{\mathrm{KL}}(\rho_{\mathrm{hist}}^{(T)} \,\|\, \rho^\star_{\epsilon_{\mathrm{relax}}=0})\),
    \(D_{\mathrm{KL}}(\rho_{\mathrm{QR}}^{(T)} \,\|\, \rho^\star_{\epsilon_{\mathrm{relax}}=0})\),
    \(D_{\mathrm{KL}}(\rho_{\mathrm{marg}}^{(T)} \,\|\, \rho^\star_{\epsilon_{\mathrm{relax}}=0})\),
    and
    \(D_{\mathrm{KL}}(\rho_{\mathrm{hist}}^{(T)} \,\|\, \rho_{\mathrm{QR}}^{(T)})\).
    These are diagnostic quantities rather than the main evaluation metric;
    they are used to understand whether mismatch comes from the theory benchmark,
    from the QR remapping, or from collapsing the joint distribution to marginals.
    Lower values indicate closer agreement.
    }
    \label{fig:proxy_all_games}
\end{figure}

% =========================================================
% Theory epsilon sensitivity
% =========================================================
\begin{figure}[t]
    \centering

    \begin{subfigure}[t]{0.32\textwidth}
        \centering
        \includegraphics[width=\linewidth]{battle_of_the_sexes_theory_eps_sensitivity_T1000.png}
        \caption{Battle of the Sexes}
    \end{subfigure}\hfill
    \begin{subfigure}[t]{0.32\textwidth}
        \centering
        \includegraphics[width=\linewidth]{prisoners_dilemma_theory_eps_sensitivity_T1000.png}
        \caption{Prisoner's Dilemma}
    \end{subfigure}\hfill
    \begin{subfigure}[t]{0.32\textwidth}
        \centering
        \includegraphics[width=\linewidth]{chicken_theory_eps_sensitivity_T1000.png}
        \caption{Chicken}
    \end{subfigure}

    \caption{
    Sensitivity of the theory benchmark to the relaxation level
    \(\epsilon_{\mathrm{relax}}\) at \(T=1000\).
    Each curve reports the held-out prediction error
    \(D_{\mathrm{KL}}(\rho_{\mathrm{future}}^{(T,H)} \,\|\, \rho^\star_{\epsilon_{\mathrm{relax}}})\)
    as \(\epsilon_{\mathrm{relax}}\) varies.
    This figure shows whether relaxing the obedience constraints improves predictive performance.
    Lower values are better.
    }
    \label{fig:theory_eps_sensitivity}
\end{figure}

\paragraph{Payoff matrices used in the code.}
The synthetic benchmark uses the following six normal-form games.

\textbf{Matching Pennies} (action order: Heads, Tails):
\[
R_1=
\begin{bmatrix}
1 & -1\\
-1 & 1
\end{bmatrix},
\qquad
R_2=
\begin{bmatrix}
-1 & 1\\
1 & -1
\end{bmatrix}.
\]

\textbf{Battle of the Sexes} (action order: Opera, Football):
\[
R_1=
\begin{bmatrix}
2 & 0\\
0 & 1
\end{bmatrix},
\qquad
R_2=
\begin{bmatrix}
1 & 0\\
0 & 2
\end{bmatrix}.
\]

\textbf{Prisoner's Dilemma} (action order: Cooperate, Defect):
\[
R_1=
\begin{bmatrix}
-1 & -3\\
0 & -2
\end{bmatrix},
\qquad
R_2=
\begin{bmatrix}
-1 & 0\\
-3 & -2
\end{bmatrix}.
\]

\textbf{Stag Hunt} (action order: Stag, Hare):
\[
R_1=
\begin{bmatrix}
4 & 0\\
3 & 2
\end{bmatrix},
\qquad
R_2=
\begin{bmatrix}
4 & 3\\
0 & 2
\end{bmatrix}.
\]

\textbf{Chicken} (action order: Swerve, Straight):
\[
R_1=
\begin{bmatrix}
0 & -1\\
1 & -10
\end{bmatrix},
\qquad
R_2=
\begin{bmatrix}
0 & 1\\
-1 & -10
\end{bmatrix}.
\]

\textbf{Rock--Paper--Scissors} (action order: Rock, Paper, Scissors):
\[
R_1=
\begin{bmatrix}
0 & -1 & 1\\
1 & 0 & -1\\
-1 & 1 & 0
\end{bmatrix},
\qquad
R_2=
\begin{bmatrix}
0 & 1 & -1\\
-1 & 0 & 1\\
1 & -1 & 0
\end{bmatrix}
=
-R_1.
\]
\newpage

\paragraph{ human-data benchmark game.}
For the Zhang-style repeated RPS benchmark, the code also includes a nonstandard RPS payoff matrix with action order
(Rock, Paper, Scissors):
\[
R_1=
\begin{bmatrix}
2 & 1 & 4\\
3 & 2 & 1\\
0 & 3 & 2
\end{bmatrix},
\qquad
R_2=
\begin{bmatrix}
2 & 3 & 0\\
1 & 2 & 3\\
4 & 1 & 2
\end{bmatrix}.
\]
This corresponds to tie payoff \(2\) each, Rock vs.\ Paper \((1,3)\), Paper vs.\ Scissors \((1,3)\), and Rock vs.\ Scissors \((4,0)\).


\newpage
\section{External Benchmark: Selten--Chmura Experimental $2\times 2$ Games}
\label{sec:selten-chmura-multi-gamma}

\subsection{Dataset and empirical target}

We evaluate the relaxed-obedience predictor on the public Selten--Chmura benchmark of completely mixed $2\times 2$ games.
Let
\[
A_1=\{U,D\},
\qquad
A_2=\{L,R\}.
\]
The benchmark contains $12$ games.
Games $1,\ldots,6$ are constant-sum and games $7,\ldots,12$ are paired nonconstant-sum variants.
The experiment was run in $54$ sessions with $16$ subjects each, and each session contained two independent subject groups.
Thus the data contain $108$ independent subject groups in total: $12$ groups for each constant-sum game and $6$ groups for each nonconstant-sum game.
Within each independent group there are four players in role $1$ and four players in role $2$, with fixed roles and random matching over $200$ periods.
Each period therefore generates four simultaneous realized two-player matches.
Hence, for one fixed game $g$ and one fixed group $j$,
\[
100 \text{ periods } \Longrightarrow 400 \text{ realized action pairs},
\qquad
200 \text{ periods } \Longrightarrow 800 \text{ realized action pairs}.
\]

The public spreadsheet does not release raw match-by-match logs.
Instead, it reports group-level relative frequencies for matrix fields $1,2,3,4$ over periods $1{:}100$, $101{:}200$, and $1{:}200$.
The documentation maps these four fields to the joint actions
\[
1\leftrightarrow (U,L),
\qquad
2\leftrightarrow (U,R),
\qquad
3\leftrightarrow (D,L),
\qquad
4\leftrightarrow (D,R).
\]
Accordingly, for each game $g$ and group $j$, the released frequencies already determine an empirical joint distribution over action pairs.
Let
\begin{align}
\rho_{\mathrm{hist},g,j}^{(100)}(a_1,a_2)
&=
\frac{C_{g,j}^{\mathrm{hist}}(a_1,a_2)}{400},
\\
\rho_{\mathrm{future},g,j}^{(100,100)}(a_1,a_2)
&=
\frac{C_{g,j}^{\mathrm{future}}(a_1,a_2)}{400},
\end{align}
where $C_{g,j}^{\mathrm{hist}}$ and $C_{g,j}^{\mathrm{future}}$ are the reconstructed first-half and second-half counts obtained by multiplying the released field frequencies by $400$.
The full-horizon empirical joint is
\[
\rho_{g,j}^{(200)}(a_1,a_2)=\frac{C_{g,j}^{(200)}(a_1,a_2)}{800}.
\]
The spreadsheet is internally consistent: for every group observation,
\[
\rho_{g,j}^{(200)} = \frac{1}{2}\rho_{\mathrm{hist},g,j}^{(100)} + \frac{1}{2}\rho_{\mathrm{future},g,j}^{(100,100)}
\]
up to numerical rounding.

The main empirical target in the static benchmark is the second-half joint distribution
$\rho_{\mathrm{future},g,j}^{(100,100)}$.
The first-half joint distribution
$\rho_{\mathrm{hist},g,j}^{(100)}$
is used only in the secondary history-to-future benchmark.
This is a group-level stationary benchmark: the theory remains a two-player static predictor, but the empirical target is the pooled distribution of realized two-player matches within one independent subject group.

\subsection{CQRE with three relaxation families}

For each game $g$, let $\bar U_1^{(g)}$ and $\bar U_2^{(g)}$ denote the original payoff matrices.
Since the relaxation parameters are measured in utility units, we normalize payoffs game by game:
\begin{equation}
\Delta_i(g)
=
\max_{a_i,\tilde a_i,a_{-i}}
\left|
\bar U_i^{(g)}(\tilde a_i,a_{-i})-\bar U_i^{(g)}(a_i,a_{-i})
\right|,
\qquad
U_i^{(g)}=\bar U_i^{(g)}/\Delta_i(g),
\quad i\in\{1,2\}.
\label{eq:selten-multigamma-normalization}
\end{equation}
This keeps the unilateral deviation structure unchanged while allowing a single grid of relaxation values to be used across games.

For a fixed game $g$, let $\rho\in\Delta(A_1\times A_2)$ denote a joint distribution over action pairs.
The relaxed-obedience feasible set is
\begin{equation}
\begin{aligned}
K_{\gamma}^{(g)}
=
\Bigl\{
\rho\in\Delta(A_1\times A_2):\;&
\sum_{a_2\in A_2}
\rho(U,a_2)
\bigl(U_1^{(g)}(D,a_2)-U_1^{(g)}(U,a_2)\bigr)
\le \gamma_U,
\\
&
\sum_{a_2\in A_2}
\rho(D,a_2)
\bigl(U_1^{(g)}(U,a_2)-U_1^{(g)}(D,a_2)\bigr)
\le \gamma_D,
\\
&
\sum_{a_1\in A_1}
\rho(a_1,L)
\bigl(U_2^{(g)}(a_1,R)-U_2^{(g)}(a_1,L)\bigr)
\le \gamma_L,
\\
&
\sum_{a_1\in A_1}
\rho(a_1,R)
\bigl(U_2^{(g)}(a_1,L)-U_2^{(g)}(a_1,R)\bigr)
\le \gamma_R
\Bigr\}.
\end{aligned}
\label{eq:selten-multigamma-feasible}
\end{equation}
The corresponding CQRE predictor is the unique maximum-entropy point in this feasible set:
\begin{equation}
\rho_{g,\gamma}^{\star}
=
\arg\min_{\rho\in K_{\gamma}^{(g)}}
\sum_{a_1,a_2}\rho(a_1,a_2)\log \rho(a_1,a_2).
\label{eq:selten-multigamma-cqre}
\end{equation}
When $\gamma=(0,0,0,0)$, this reduces to the exact maximum-entropy correlated-equilibrium benchmark.
For any fixed $\gamma$, solving \eqref{eq:selten-multigamma-cqre} uses only the payoff matrix; the human data are used only to evaluate the fit of the resulting predictor or to select a common relaxation parameterization.

We study three nested relaxation families:
\begin{align}
\text{scalar:} &\qquad
\gamma_U=\gamma_D=\gamma_L=\gamma_R=\epsilon_{\mathrm{relax}},
\label{eq:selten-scalar-gamma}
\\
\text{per-player:} &\qquad
\gamma_U=\gamma_D=\epsilon_1,
\qquad
\gamma_L=\gamma_R=\epsilon_2,
\label{eq:selten-player-gamma}
\\
\text{per-action:} &\qquad
\gamma=(\gamma_U,\gamma_D,\gamma_L,\gamma_R).
\label{eq:selten-action-gamma}
\end{align}
The scalar family is the direct analogue of the single-$\epsilon_{\mathrm{relax}}$ specification in the main text.
The per-player family allows the two roles to have different effective relaxation levels.
The per-action family is the most flexible and allows the slack to depend on the recommended action itself.

A key structural property of the current formulation is invariance to additive row/column shifts that preserve deviation differences.
If
\[
U_1'(a_1,a_2)=U_1(a_1,a_2)+c(a_2),
\qquad
U_2'(a_1,a_2)=U_2(a_1,a_2)+d(a_1),
\]
then every unilateral deviation difference is unchanged, hence the feasible set and the optimizer are unchanged:
\[
K_{\gamma}(U_1',U_2')=K_{\gamma}(U_1,U_2),
\qquad
\rho_{\gamma}^{\star}(U_1',U_2')=\rho_{\gamma}^{\star}(U_1,U_2).
\]
This matters for Selten--Chmura because games $7,\ldots,12$ are constructed from games $1,\ldots,6$ by exactly such additive shifts.
Therefore, for every one of the three CQRE families above, the current formulation makes identical predictions within each pair $(1,7),\ldots,(6,12)$.

\subsection{Experiment design}

We run two evaluation layers.

\paragraph{(i) Static payoff-only benchmark on games $1$--$6$.}
The main benchmark uses the constant-sum games only.
For each held-out constant-sum game $g\in\{1,\ldots,6\}$, we fit a \emph{global} relaxation parameterization on the other five constant-sum games and evaluate it on all groups of the held-out game.
For a CQRE family $\Gamma$, the selected parameter is
\begin{equation}
\hat\gamma_{\Gamma}^{(-g)}
=
\arg\min_{\gamma\in\Gamma}
\frac{1}{|\mathcal T_g|}
\sum_{(g',j)\in \mathcal T_g}
D_{\mathrm{KL}}
\Bigl(
\rho_{\mathrm{future},g',j}^{(100,100)}
\,\|\,
\rho_{g',\gamma}^{\star}
\Bigr),
\label{eq:selten-gamma-cv}
\end{equation}
where $\mathcal T_g$ denotes the training observations from the other five constant-sum games.
The candidate grid is
\[
\{0,
0.005,
0.01,
0.02,
0.05,
0.1,
0.2\}.
\]
The baselines are:
\begin{itemize}
    \item mixed Nash product $\rho_g^{\mathrm{Nash}}$;
    \item logit-QRE product $\rho_{g,\beta}^{\mathrm{QRE}}$, with one global $\beta$ selected analogously by leave-one-game-out cross-validation;
    \item exact CQRE $\rho_{g,(0,0,0,0)}^{\star}$;
    \item relaxed CQRE under the scalar, per-player, and per-action families.
\end{itemize}
All models are scored by
\begin{equation}
\mathrm{KL}_{\mathrm{pred}}(Q;100,100)
=
D_{\mathrm{KL}}
\Bigl(
\rho_{\mathrm{future},g,j}^{(100,100)}
\,\|\,
Q
\Bigr).
\label{eq:selten-multigamma-kl}
\end{equation}

\paragraph{(ii) History-to-future benchmark on games $1$--$6$.}
To stay close to the predictive setup in the main experiment section, we also use the first-half frequencies as history and the second-half frequencies as hold-out future.
For each group observation we compare the same future target $\rho_{\mathrm{future},g,j}^{(100,100)}$ against:
\begin{itemize}
    \item the direct history joint $\rho_{\mathrm{hist},g,j}^{(100)}$;
    \item the product of first-half empirical marginals $\rho_{\mathrm{marg},g,j}^{(100)}$;
    \item a history-based unconditional QR product $\rho_{\mathrm{QR},g,j}^{(100)}$;
    \item the same payoff-only models used in the static benchmark.
\end{itemize}
For the history-based QR baseline we fit a single global inverse-temperature parameter $\beta_{\mathrm{hist}}$ on the training games.

\paragraph{(iii) Paired nonconstant-sum stress test on games $7$--$12$.}
After refitting the best scalar, per-player, and per-action CQRE parameters on all constant-sum games $1$--$6$, we carry them unchanged to the paired nonconstant-sum games $7$--$12$.
This is a pure out-of-family stress test of the invariance built into the current formulation.
Since the model is pair-invariant by construction, these games reveal whether human behavior is also approximately invariant under the same additive payoff shifts.

\subsection{Implementation checks and reproducibility}

We verified the code and results in four ways.
First, rerunning the full script from scratch on the public spreadsheet reproduced the archived CSV and JSON outputs exactly.
Second, the benchmark structure is internally consistent: all $108$ group observations satisfy the expected $400/400/800$ count identities for periods $1{:}100$, $101{:}200$, and $1{:}200$.
Third, the reconstructed full-horizon frequencies agree with the average of the two half-windows up to machine precision.
Fourth, the CQRE solver is numerically feasible across the full cached grid: the largest obedience violation over all solved CQRE instances is $7.78\times 10^{-14}$, and the largest difference between paired-game CQRE predictions over the full cache is $1.51\times 10^{-11}$.
Thus the numerical results below are fully reproducible and internally consistent.

\subsection{Selected parameters}

Table~\ref{tab:selten-multigamma-params} reports the parameters selected after refitting on all constant-sum games $1$--$6$.
The best scalar relaxation is $\epsilon_{\mathrm{relax}}=0.01$.
Allowing different relaxation levels by role improves the fit and yields $(\epsilon_1,\epsilon_2)=(0.02,0.005)$.
The best per-action specification is $(\gamma_U,\gamma_D,\gamma_L,\gamma_R)=(0.02,0.02,0,0.005)$.
For comparison, the best global logit-QRE baseline uses $\beta=11.221$ in the static benchmark and $\beta_{\mathrm{hist}}=6.220$ in the history-based QR baseline.

\begin{table}[t]
\centering
\caption{Selected global parameters after refitting on constant-sum games $1$--$6$.}
\label{tab:selten-multigamma-params}
\begin{tabular}{lll}
\toprule
Model family & Selected parameter(s) & Training mean KL \\
\midrule
Scalar CQRE & $\epsilon_{\mathrm{relax}}=0.01$ & 0.0382 \\
Per-player CQRE & $(\epsilon_1,\epsilon_2)=(0.02,0.005)$ & 0.0366 \\
Per-action CQRE & $(\gamma_U,\gamma_D,\gamma_L,\gamma_R)=(0.02,0.02,0,0.005)$ & 0.0361 \\
Logit QRE baseline & $\beta=11.221$ & 0.0303 \\
History-QR baseline & $\beta_{\mathrm{hist}}=6.220$ & 0.1153 \\
\bottomrule
\end{tabular}
\end{table}

\subsection{Results on constant-sum games $1$--$6$}

Table~\ref{tab:selten-multigamma-static} reports the main static payoff-only benchmark.
The strongest model is global logit QRE with mean KL $0.0334$.
Among the CQRE variants, the per-player family performs best, followed by the per-action family and then the scalar family.
All three relaxed CQRE families substantially improve on exact CQRE.
In this benchmark exact CQRE is numerically indistinguishable from mixed Nash: both have mean KL $0.0832$.

\begin{table}[t]
\centering
\caption{Constant-sum games $1$--$6$: static payoff-only evaluation against $\rho_{\mathrm{future},g,j}^{(100,100)}$. Lower is better.}
\label{tab:selten-multigamma-static}
\begin{tabular}{lcccc}
\toprule
Model & $n$ & Mean KL & Median KL & SE \\
\midrule
Logit QRE product & 72 & 0.0334 & 0.0202 & 0.0044 \\
CQRE, per-player & 72 & 0.0414 & 0.0239 & 0.0056 \\
CQRE, per-action & 72 & 0.0446 & 0.0226 & 0.0061 \\
CQRE, scalar & 72 & 0.0469 & 0.0256 & 0.0064 \\
Exact CQRE & 72 & 0.0832 & 0.0436 & 0.0120 \\
Mixed Nash product & 72 & 0.0832 & 0.0436 & 0.0120 \\
\bottomrule
\end{tabular}
\end{table}

Table~\ref{tab:selten-multigamma-predictive} reports the secondary history-to-future benchmark.
As expected in repeated interaction with feedback, the empirical history baselines are strongest.
The product of first-half marginals achieves the best fit, closely followed by the first-half joint itself.
Among payoff-only models, the ordering is the same as in the static benchmark: logit QRE first, then per-player CQRE, then per-action CQRE, then scalar CQRE, and finally exact CQRE / Nash.

\begin{table}[t]
\centering
\caption{Constant-sum games $1$--$6$: history-to-future evaluation. Lower is better.}
\label{tab:selten-multigamma-predictive}
\begin{tabular}{lcccc}
\toprule
Model & $n$ & Mean KL & Median KL & SE \\
\midrule
History marginal product & 72 & 0.0173 & 0.0103 & 0.0022 \\
History joint & 72 & 0.0180 & 0.0102 & 0.0023 \\
Logit QRE product & 72 & 0.0334 & 0.0202 & 0.0044 \\
CQRE, per-player & 72 & 0.0414 & 0.0239 & 0.0056 \\
CQRE, per-action & 72 & 0.0446 & 0.0226 & 0.0061 \\
CQRE, scalar & 72 & 0.0469 & 0.0256 & 0.0064 \\
Exact CQRE & 72 & 0.0832 & 0.0436 & 0.0120 \\
History QR product & 72 & 0.1255 & 0.0727 & 0.0160 \\
\bottomrule
\end{tabular}
\end{table}

\begin{figure}[t]
    \centering
    \includegraphics[width=0.92\linewidth]{plots/constant_sum_static_plot.png}
    \caption{Constant-sum games $1$--$6$: mean KL in the main static payoff-only benchmark.}
    \label{fig:selten-multigamma-static}
\end{figure}

\begin{figure}[t]
    \centering
    \includegraphics[width=0.92\linewidth]{plots/constant_sum_predictive_plot.png}
    \caption{Constant-sum games $1$--$6$: mean KL in the history-to-future benchmark.}
    \label{fig:selten-multigamma-predictive}
\end{figure}

\subsection{Results on paired nonconstant-sum games $7$--$12$}

Table~\ref{tab:selten-multigamma-paired} reports the paired nonconstant-sum stress test using the parameters selected on games $1$--$6$.
Here the ranking changes.
All three relaxed CQRE families outperform global logit QRE, and the best performer is now the per-player family, closely followed by the per-action family.
Thus, although the paired games are a stress test for the invariance built into the current formulation, the relaxed CQRE families remain competitive and in fact dominate the static logit-QRE baseline on these six games.

\begin{table}[t]
\centering
\caption{Paired nonconstant-sum games $7$--$12$: static payoff-only evaluation using parameters fit on constant-sum games $1$--$6$. Lower is better.}
\label{tab:selten-multigamma-paired}
\begin{tabular}{lcccc}
\toprule
Model & $n$ & Mean KL & Median KL & SE \\
\midrule
CQRE, per-player & 36 & 0.0255 & 0.0175 & 0.0036 \\
CQRE, per-action & 36 & 0.0260 & 0.0170 & 0.0036 \\
CQRE, scalar & 36 & 0.0299 & 0.0182 & 0.0040 \\
Logit QRE product & 36 & 0.0376 & 0.0282 & 0.0059 \\
Exact CQRE & 36 & 0.0898 & 0.0397 & 0.0187 \\
Mixed Nash product & 36 & 0.0898 & 0.0397 & 0.0187 \\
\bottomrule
\end{tabular}
\end{table}

The secondary history-to-future evaluation on games $7$--$12$ shows a similar pattern.
The per-player and per-action CQRE families again outperform the static logit-QRE baseline and are competitive with the history baselines.
The best mean KL is $0.0255$ for per-player CQRE, compared with $0.0262$ for the first-half marginal-product baseline and $0.0274$ for the first-half joint baseline.

The paired-game diagnostic reveals where the current formulation is limited.
Although the model is exactly pair-invariant by construction, the empirical mean second-half joint distributions are not.
The $\ell_1$ shift between the mean future joints of paired games ranges from $0.0354$ for pair $(6,12)$ to $0.2075$ for pair $(1,7)$.
Thus the data contain payoff-level effects that are invisible to the current deviation-difference-based CQRE constraints.

\begin{figure}[t]
    \centering
    \includegraphics[width=0.92\linewidth]{plots/paired_static_plot.png}
    \caption{Paired nonconstant-sum games $7$--$12$: mean KL in the static payoff-only stress test.}
    \label{fig:selten-multigamma-paired-static}
\end{figure}

\begin{figure}[t]
    \centering
    \includegraphics[width=0.92\linewidth]{plots/paired_predictive_plot.png}
    \caption{Paired nonconstant-sum games $7$--$12$: mean KL in the history-to-future stress test.}
    \label{fig:selten-multigamma-paired-predictive}
\end{figure}

\begin{figure}[t]
    \centering
    \includegraphics[width=0.72\linewidth]{plots/pair_shift_plot.png}
    \caption{Empirical shift between paired mean future joint distributions for $(g,g+6)$.}
    \label{fig:selten-multigamma-pair-shift}
\end{figure}

\subsection{Interpretation}

This benchmark yields four main conclusions.
First, exact CE-style prediction is too rigid on these data: exact CQRE is numerically equivalent to mixed Nash and fits poorly.
Second, a small global scalar relaxation improves fit substantially, but allowing role-specific or action-specific relaxation improves it further.
Third, on the main constant-sum benchmark the best static payoff-only model remains global logit QRE, whereas on the paired nonconstant-sum stress test the relaxed CQRE families outperform static logit QRE.
Fourth, the paired games isolate a genuine limitation of the current formulation: because the constraints depend only on unilateral deviation differences, additive payoff shifts that leave those differences unchanged do not affect the CQRE prediction, even though they can move human behavior appreciably.

The strongest claim supported by this benchmark is therefore not that CQRE dominates all alternatives uniformly.
Rather, the evidence shows that exact CE/Nash is too rigid, that structured relaxation materially improves fit, and that the Selten--Chmura paired-game construction reveals exactly which invariances the current formulation imposes.



\end{document}
