# Supplementary material for: Correlated Quantal Response Equilibrium: A New Equilibrium Notion for Human-AI Strategic Interactions
Source: arXiv:2610.29020 source file (2026-10-21)
Supplement: Supplementary file 5 [file appendix-llm-roundrobin.tex]

\subsection{Frontier GPT round-robin details}
\label{appendix:gpt-roundrobin-details}

This appendix gives additional detail for the GPT round-robin reported in Section~\ref{subsec:gpt-roundrobin-results}.  Each model pair is evaluated on the weighted rock--paper--scissors game in~\eqref{eq:weighted-rps-payoff-main}.  For every completed pair, the empirical target $\widehat p$ is the $9$-cell empirical joint distribution over canonical actions $(R,P,S)^2$ after undoing the per-match random relabeling of displayed actions.  The fitted models are the mixed Nash product, logit QRE product, exact CQRE, CQRE scalar, CQRE per-player, and CQRE per-action.  Parameters are fit separately for each model pair by minimizing $D_{\mathrm{KL}}(\widehat p\|p_\theta)$.  Bootstrap intervals are computed by multinomial resampling of the empirical $9$-cell joint with $N=200$ and $B=1000$ replicates, keeping the fitted model distributions fixed.

\begin{table}[H]
\centering
\scriptsize
\resizebox{\textwidth}{!}{%
\begin{tabular}{lrrrrrr}
\toprule
Pair & Nash & Logit QRE & Exact CQRE & CQRE scalar & CQRE per-player & CQRE per-action \\
\midrule
gpt-4o-mini vs gpt-5         & 0.1201 & 0.0910 & 0.1201 & 0.1104 & 0.1064 & 0.0907 \\
gpt-4o vs gpt-5              & 0.1453 & 0.1348 & 0.1453 & 0.1453 & 0.1453 & 0.1380 \\
gpt-4.1 vs gpt-5             & 0.2069 & 0.1693 & 0.2069 & 0.2069 & 0.2048 & 0.1759 \\
gpt-4.1 vs gpt-4.1-mini      & 0.2183 & 0.0815 & 0.2183 & 0.0862 & 0.0706 & 0.0706 \\
gpt-4o vs gpt-5-mini         & 0.2425 & 0.0849 & 0.2425 & 0.1272 & 0.1272 & 0.1091 \\
gpt-4.1 vs gpt-5-mini        & 0.2799 & 0.1372 & 0.2799 & 0.1910 & 0.1738 & 0.1438 \\
gpt-4o-mini vs gpt-5-mini    & 0.2843 & 0.0958 & 0.2843 & 0.1453 & 0.1453 & 0.1292 \\
gpt-4.1-mini vs gpt-5        & 0.3153 & 0.2364 & 0.3153 & 0.2856 & 0.2846 & 0.2314 \\
gpt-4.1-mini vs gpt-4o       & 0.3420 & 0.1234 & 0.3420 & 0.1477 & 0.1324 & 0.1218 \\
gpt-4.1 vs gpt-4o            & 0.3438 & 0.2383 & 0.3438 & 0.2789 & 0.2760 & 0.2176 \\
gpt-4.1 vs gpt-4o-mini       & 0.3938 & 0.2468 & 0.3938 & 0.2690 & 0.2674 & 0.2274 \\
gpt-4.1-mini vs gpt-4o-mini  & 0.4010 & 0.1517 & 0.4010 & 0.1722 & 0.1722 & 0.1715 \\
gpt-4.1-mini vs gpt-5-mini   & 0.4503 & 0.1928 & 0.4503 & 0.2492 & 0.2438 & 0.2308 \\
gpt-4.1 vs gpt-4.1           & 0.4551 & 0.3979 & 0.4551 & 0.4180 & 0.4165 & 0.3653 \\
gpt-5 vs gpt-5-mini          & 0.6084 & 0.4694 & 0.6084 & 0.5580 & 0.5551 & 0.4817 \\
gpt-4.1-mini vs gpt-4.1-mini & 0.6114 & 0.3372 & 0.6114 & 0.3811 & 0.3196 & 0.3196 \\
gpt-4o-mini vs gpt-4o-mini   & 0.6278 & 0.3990 & 0.6278 & 0.3990 & 0.3990 & 0.3885 \\
gpt-4o vs gpt-4o             & 0.6373 & 0.6384 & 0.6373 & 0.5472 & 0.5472 & 0.4978 \\
gpt-4o vs gpt-4o-mini        & 0.6830 & 0.5027 & 0.6830 & 0.5027 & 0.5027 & 0.4758 \\
gpt-5-mini vs gpt-5-mini     & 0.7987 & 0.5385 & 0.7987 & 0.6378 & 0.6117 & 0.5458 \\
\bottomrule
\end{tabular}}
\caption{GPT round-robin point estimates: $D_{\mathrm{KL}}(\widehat p\|p_{\theta^\star})$ for each model pair and equilibrium notion.  Lower is better.}
\label{tab:gpt-pairs-kl-appendix}
\end{table}

\begin{figure}[H]
\centering
\begin{subfigure}[t]{0.48\textwidth}
\centering
\includegraphics[width=\linewidth]{fit_models_grouped_bar.pdf}
\caption{All six notions per pair.}
\label{fig:gpt-grouped-bar-appendix}
\end{subfigure}\hfill
\begin{subfigure}[t]{0.48\textwidth}
\centering
\includegraphics[width=\linewidth]{fit_models_paired_lines.pdf}
\caption{Parallel coordinates by pair.}
\label{fig:gpt-paired-lines-appendix}
\end{subfigure}
\caption{Additional GPT round-robin visualizations.  The grouped bars display all six equilibrium notions for every pair with bootstrap whiskers.  The parallel-coordinate plot shows the characteristic drop from Nash/exact CQRE to logit QRE and relaxed CQRE.}
\label{fig:gpt-additional-fits-appendix}
\end{figure}

\begin{figure}[H]
\centering
\includegraphics[width=0.70\textwidth]{cqre_per_action_heatmap.pdf}
\caption{Heatmap of KL to CQRE per-action across GPT model pairs.  The missing diagonal entry corresponds to \textsf{gpt-5} self-play, which timed out during generation.}
\label{fig:gpt-cqre-heatmap-appendix}
\end{figure}
