# Supplementary material for: Correlated Quantal Response Equilibrium: A New Equilibrium Notion for Human-AI Strategic Interactions
Source: arXiv:2610.29020 source file (2026-10-21)
Supplement: Supplementary file 6 [file appendix-numerical-experiments.tex]

\section{Additional Numerical Details}
\label{appendix:numerical-details}

\subsection{Synthetic fictitious-play benchmark}
\label{appendix:synthetic-details}

The synthetic benchmark uses six finite two-player normal-form games: matching pennies, rock--paper--scissors, prisoner's dilemma, battle of the sexes, chicken, and stag hunt.  For each game we generate one long trajectory using a stochastic smoothed fictitious-play process.  At time $t$, the simulator stores exponentially smoothed beliefs $FP_{1,t}\in\Delta(A_1)$ and $FP_{2,t}\in\Delta(A_2)$, initialized uniformly.  It samples proxy actions from these beliefs,
\begin{equation}
    a_2'\sim FP_{2,t},\qquad a_1'\sim FP_{1,t},
\end{equation}
and then each player plays a soft best response to the proxy action,
\begin{equation}
    a_{1,t}\sim \mathrm{SoftBR}_1(\cdot\mid a_2'),
    \qquad
    a_{2,t}\sim \mathrm{SoftBR}_2(\cdot\mid a_1'),
\end{equation}
where
\begin{equation}
    \mathrm{SoftBR}_1(a_1\mid a_2')=
    \frac{\exp(U_1(a_1,a_2')/\tau_1)}{\sum_{\tilde a_1}\exp(U_1(\tilde a_1,a_2')/\tau_1)},
\end{equation}
and analogously for player 2.  Beliefs are updated by exponential moving average,
\begin{equation}
    FP_{1,t+1}=\alpha FP_{1,t}+(1-\alpha)e_{a_{1,t}},
    \qquad
    FP_{2,t+1}=\alpha FP_{2,t}+(1-\alpha)e_{a_{2,t}}.
\end{equation}
Conditional on $(FP_{1,t},FP_{2,t})$, the one-step joint distribution factorizes.  Hence this simulator is useful as a controlled diagnostic, but it does not directly generate strong within-round correlation.

For each history length $T\in\{100,300,1000,3000,10000\}$, the history empirical joint and future empirical joint are
\begin{equation}
    \rho_{\mathrm{hist}}^{(T)}(a_1,a_2)=\frac{1}{T}\sum_{t=1}^T \mathbf 1\{(a_{1,t},a_{2,t})=(a_1,a_2)\},
\end{equation}
\begin{equation}
    \rho_{\mathrm{future}}^{(T,H)}(a_1,a_2)=\frac{1}{H}\sum_{t=T+1}^{T+H} \mathbf 1\{(a_{1,t},a_{2,t})=(a_1,a_2)\}.
\end{equation}
The four synthetic predictors are: (i) the direct history joint $\rho_{\mathrm{hist}}^{(T)}$; (ii) the product of smoothed empirical history marginals; (iii) an unconditional QR product induced from the history marginals; and (iv) the exact or relaxed CQRE predictor computed from the stage-game payoff matrix.  The main score is $D_{\mathrm{KL}}(\rho_{\mathrm{future}}^{(T,H)}\|Q)$.

\begin{figure}[H]
    \centering
    \begin{subfigure}[t]{0.32\textwidth}
        \centering\includegraphics[width=\linewidth]{matching_pennies_prediction.png}
        \caption{Matching pennies.}
    \end{subfigure}\hfill
    \begin{subfigure}[t]{0.32\textwidth}
        \centering\includegraphics[width=\linewidth]{rock_paper_scissors_prediction.png}
        \caption{Rock--paper--scissors.}
    \end{subfigure}\hfill
    \begin{subfigure}[t]{0.32\textwidth}
        \centering\includegraphics[width=\linewidth]{prisoners_dilemma_prediction.png}
        \caption{Prisoner's dilemma.}
    \end{subfigure}

    \vspace{0.6em}
    \begin{subfigure}[t]{0.32\textwidth}
        \centering\includegraphics[width=\linewidth]{battle_of_the_sexes_prediction.png}
        \caption{Battle of the sexes.}
    \end{subfigure}\hfill
    \begin{subfigure}[t]{0.32\textwidth}
        \centering\includegraphics[width=\linewidth]{chicken_prediction.png}
        \caption{Chicken.}
    \end{subfigure}\hfill
    \begin{subfigure}[t]{0.32\textwidth}
        \centering\includegraphics[width=\linewidth]{stag_hunt_prediction.png}
        \caption{Stag hunt.}
    \end{subfigure}
    \caption{Held-out KL prediction error on synthetic trajectories generated by smoothed fictitious play. Lower is better.}
    \label{fig:fictitious-play-prediction}
\end{figure}

\begin{figure}[H]
    \centering
    \begin{subfigure}[t]{0.32\textwidth}
        \centering\includegraphics[width=\linewidth]{matching_pennies_proxy.png}
        \caption{Matching pennies.}
    \end{subfigure}\hfill
    \begin{subfigure}[t]{0.32\textwidth}
        \centering\includegraphics[width=\linewidth]{rock_paper_scissors_proxy.png}
        \caption{Rock--paper--scissors.}
    \end{subfigure}\hfill
    \begin{subfigure}[t]{0.32\textwidth}
        \centering\includegraphics[width=\linewidth]{prisoners_dilemma_proxy.png}
        \caption{Prisoner's dilemma.}
    \end{subfigure}

    \vspace{0.6em}
    \begin{subfigure}[t]{0.32\textwidth}
        \centering\includegraphics[width=\linewidth]{battle_of_the_sexes_proxy.png}
        \caption{Battle of the sexes.}
    \end{subfigure}\hfill
    \begin{subfigure}[t]{0.32\textwidth}
        \centering\includegraphics[width=\linewidth]{chicken_proxy.png}
        \caption{Chicken.}
    \end{subfigure}\hfill
    \begin{subfigure}[t]{0.32\textwidth}
        \centering\includegraphics[width=\linewidth]{stag_hunt_proxy.png}
        \caption{Stag hunt.}
    \end{subfigure}
    \caption{Proxy diagnostics for the synthetic fictitious-play benchmark. Lower values indicate closer agreement between the empirical history distribution and the corresponding benchmark object.}
    \label{fig:fictitious-play-proxy}
\end{figure}

\begin{figure}[H]
    \centering
    \begin{subfigure}[t]{0.32\textwidth}
        \centering\includegraphics[width=\linewidth]{battle_of_the_sexes_theory_eps_sensitivity_T1000.png}
        \caption{Battle of the sexes.}
    \end{subfigure}\hfill
    \begin{subfigure}[t]{0.32\textwidth}
        \centering\includegraphics[width=\linewidth]{prisoners_dilemma_theory_eps_sensitivity_T1000.png}
        \caption{Prisoner's dilemma.}
    \end{subfigure}\hfill
    \begin{subfigure}[t]{0.32\textwidth}
        \centering\includegraphics[width=\linewidth]{chicken_theory_eps_sensitivity_T1000.png}
        \caption{Chicken.}
    \end{subfigure}
    \caption{Sensitivity of the synthetic theory benchmark to the relaxation level in three representative games. Lower is better.}
    \label{fig:fictitious-play-sensitivity}
\end{figure}

\subsection{Selten--Chmura benchmark and data construction}
\label{appendix:selten-dataset}

The Selten--Chmura benchmark was collected in $54$ laboratory sessions with $16$ human subjects per session, for a total of $864$ participants.  Only one game was played in each session.  Each session contained two independent subject groups.  Each independent subject group consisted of four player-1 subjects and four player-2 subjects with fixed roles, random matching, and $200$ periods of interaction.  Hence each group generates $4$ realized two-player matches per period and therefore contributes $800$ realized action pairs over the full experiment.  The public spreadsheet reports relative frequencies for the four matrix cells over periods $1{:}100$, $101{:}200$, and $1{:}200$.  For games $1$--$6$, there are $12$ independent subject groups per game.  The data documentation maps fields $1,2,3,4$ to the joint actions $(U,L),(U,R),(D,L),(D,R)$.

The released spreadsheet does not provide raw match-by-match logs.  Instead, it reports group-level relative frequencies for the four joint-action cells.  Because every group contributes the same number of realized matches, pooling full-horizon empirical counts is equivalent to averaging the reported full-horizon relative frequencies across the $12$ groups for the same game.

\subsection{Construction of the empirical and theoretical distributions}
\label{appendix:construction-details}

For each game $g\in\{1,\ldots,6\}$, the empirical target is the full-horizon game-level joint distribution in~\eqref{eq:empirical-joint-main}.  The mixed Nash product benchmark is obtained from the unique mixed Nash equilibrium of the $2\times2$ game.  If
\begin{equation}
U_1 = \begin{pmatrix} a & b \\ c & d \end{pmatrix},
\qquad
U_2 = \begin{pmatrix} e & f \\ g & h \end{pmatrix},
\end{equation}
then the equilibrium mixing probabilities are given by indifference as
\begin{equation}
q_L = \frac{d-b}{a-b-c+d},
\qquad
p_U = \frac{h-g}{e-f-g+h},
\end{equation}
and the Nash benchmark is the product joint
\begin{equation}
\rho_g^{\mathrm{Nash}} =
\begin{pmatrix}
 p_U q_L, & p_U(1-q_L), & (1-p_U)q_L, & (1-p_U)(1-q_L)
\end{pmatrix}.
\end{equation}
For the logit QRE benchmark, we solve the standard fixed-point equations for a given rationality parameter $\beta$ and then form the corresponding product joint.  In the reported experiment, $\beta$ is fit independently for each game by minimizing $D_{\mathrm{KL}}(\widehat\rho_g\,\|\,\rho^{\mathrm{QRE}}_{g,\beta})$ over $\beta\in[0,20]$.

For exact CQRE, we solve the maximum-entropy correlated-equilibrium problem with zero relaxation.  For relaxed CQRE, we solve the same entropy minimization problem over the relaxed obedience set.  The implementation uses the joint distribution over the four action cells as the optimization variable and enforces the simplex constraint together with the four linear obedience constraints.  The payoffs are normalized game by game by each player's maximum unilateral deviation scale before the relaxation parameters are fit.

\subsection{Selten--Chmura bootstrap intervals by game}
\label{appendix:selten-per-game-ci}

Table~\ref{tab:first6-per-game-ci} reports the per-game bootstrap confidence intervals.  Each entry is the full-data KL followed by a $95\%$ bootstrap interval.  The bootstrap resamples independent subject groups within each game and keeps the full-data fitted model distributions fixed.

\begin{table}[H]
\centering
\scriptsize
\resizebox{\textwidth}{!}{%
\begin{tabular}{lcccccc}
\toprule
Game & Nash & Exact CQRE & Logit QRE product & CQRE scalar & CQRE per-player & CQRE per-action \\
\midrule
1 & 0.1910 [0.1298, 0.2751] & 0.1910 [0.1298, 0.2751] & 0.0183 [0.0076, 0.0431] & 0.0056 [0.0040, 0.0173] & 0.0019 [0.0004, 0.0133] & 0.0019 [0.0004, 0.0133] \\
2 & 0.0947 [0.0634, 0.1369] & 0.0947 [0.0634, 0.1369] & 0.0053 [0.0013, 0.0155] & 0.0068 [0.0016, 0.0182] & 0.0051 [0.0006, 0.0178] & 0.0051 [0.0006, 0.0178] \\
3 & 0.0952 [0.0626, 0.1378] & 0.0952 [0.0626, 0.1378] & 0.0002 [0.0001, 0.0064] & 0.0356 [0.0211, 0.0574] & 0.0347 [0.0195, 0.0570] & 0.0270 [0.0146, 0.0464] \\
4 & 0.0344 [0.0243, 0.0484] & 0.0344 [0.0243, 0.0484] & 0.0002 [0.0001, 0.0044] & 0.0147 [0.0065, 0.0271] & 0.0147 [0.0072, 0.0257] & 0.0102 [0.0051, 0.0196] \\
5 & 0.0132 [0.0082, 0.0247] & 0.0132 [0.0082, 0.0247] & 0.0011 [0.0004, 0.0090] & 0.0062 [0.0036, 0.0169] & 0.0044 [0.0019, 0.0167] & 0.0035 [0.0015, 0.0158] \\
6 & 0.0039 [0.0021, 0.0075] & 0.0039 [0.0021, 0.0075] & 0.0021 [0.0006, 0.0061] & 0.0017 [0.0008, 0.0042] & 0.0008 [0.0002, 0.0030] & 0.0008 [0.0003, 0.0029] \\
\bottomrule
\end{tabular}}
\caption{Per-game Selten--Chmura bootstrap intervals.  Each cell reports full-data KL followed by a $95\%$ bootstrap confidence interval.}
\label{tab:first6-per-game-ci}
\end{table}

\subsection{Selected per-game parameters}
\label{appendix:selten-parameters}

Table~\ref{tab:first6-selected-parameters} reports the fitted per-game QRE parameter together with the selected CQRE relaxation parameters for each of the three CQRE families.

\begin{table}[H]
\centering
\begin{tabular}{lcccccccc}
\toprule
Game & $\beta_{\mathrm{QRE}}$ & $\epsilon$ & $\epsilon_1$ & $\epsilon_2$ & $\gamma_U$ & $\gamma_D$ & $\gamma_L$ & $\gamma_R$ \\
\midrule
1 & 1.2293 & 0.010 & 0.020 & 0.000 & 0.020 & 0.000 & 0.000 & 0.000 \\
2 & 0.5726 & 0.050 & 0.050 & 0.020 & 0.050 & 0.000 & 0.020 & 0.000 \\
3 & 1.1997 & 0.020 & 0.020 & 0.010 & 0.020 & 0.000 & 0.000 & 0.020 \\
4 & 1.1007 & 0.020 & 0.020 & 0.010 & 0.005 & 0.000 & 0.000 & 0.050 \\
5 & 1.2585 & 0.010 & 0.020 & 0.005 & 0.020 & 0.000 & 0.000 & 0.010 \\
6 & 1.3271 & 0.010 & 0.020 & 0.000 & 0.020 & 0.000 & 0.000 & 0.005 \\
\bottomrule
\end{tabular}
\caption{Selected per-game QRE and CQRE fitting parameters for Selten--Chmura constant-sum games $1$--$6$.}
\label{tab:first6-selected-parameters}
\end{table}

\subsection{LLM weighted-RPS details}
\label{appendix:llm-details}

The LLM experiment uses a local MLX implementation of \texttt{mlx-community/Qwen2.5-3B-Instruct-4bit}.  Each match is a fresh one-shot prompt.  The row and column players both observe the full payoff matrix, are told their role, and output a single action.  In the shared-signal condition, both prompts include the same public signal before the one-shot decision.  The displayed action labels are randomized and mapped back to the canonical RPS actions after generation.

The reported full-data fit uses $200$ one-shot matches and the weighted RPS payoff matrices in Section~\ref{subsec:llm-rps-results}.  The bootstrap intervals in Table~\ref{tab:llm-rps-ci} resample one-shot match rows.  The fitted QRE parameter is $\beta=0.1026$.  The selected scalar CQRE relaxation is $\epsilon=0.1$; the selected per-player relaxation is $(0.2,0.1)$; and the selected per-action relaxation is $(0,0,0.1,0.005,0.2,0.1)$, with one slack for each recommended action of each player.
