# Supplementary material for: Correlated Quantal Response Equilibrium: A New Equilibrium Notion for Human-AI Strategic Interactions
Source: arXiv:2610.29020 source file (2026-10-21)
Supplement: Supplementary file 7 [file appendix-proofs.tex]

% Intentionally left empty for now. Existence and uniqueness proofs are in the main text.
