# Supplementary material for: Correlated Quantal Response Equilibrium: A New Equilibrium Notion for Human-AI Strategic Interactions
Source: arXiv:2610.29020 source file (2026-10-21)
Supplement: Supplementary file 8 [file sm_n3_ci.tex]

{\scriptsize\setlength{\tabcolsep}{2.5pt}\renewcommand{\arraystretch}{1.05}
\begin{longtable}{lrrrrrr}
\caption{Per-pair mean KL with 95\,\% bootstrap CI for game \texttt{sm\_n3}. Each cell is ``mean\,[lo,\,hi]'' in nats. Pairs sorted ascending by CQRE-pa mean. Boldface marks the lowest-mean equilibrium notion in each row.}\label{tab:appendix_ci_sm_n3}\\
\toprule
Model pair & Nash & Logit-QRE & Exact CQRE & CQRE sc. & CQRE pp. & CQRE-pa \\
\midrule
\endfirsthead
\multicolumn{7}{l}{\textit{(continued)}}\\
\toprule
Model pair & Nash & Logit-QRE & Exact CQRE & CQRE sc. & CQRE pp. & CQRE-pa \\
\midrule
\endhead
\bottomrule
\endfoot
gpt-4o vs gpt-4o-mini & 1.70[1.47,1.95] & 15.36[13.86,16.88] & 1.33[1.09,1.59] & 0.20[0.13,0.27] & 0.19[0.13,0.25] & \textbf{0.19[0.13,0.25]} \\
gpt-4o vs gpt-4o & 2.00[1.75,2.25] & 13.72[12.29,15.20] & 1.40[1.14,1.65] & 0.28[0.21,0.37] & 0.28[0.21,0.37] & \textbf{0.26[0.19,0.35]} \\
gpt-4.1-mini vs gpt-4o-mini & 1.48[1.25,1.70] & 16.38[14.87,18.00] & 1.21[0.99,1.46] & 0.29[0.24,0.35] & 0.28[0.23,0.34] & \textbf{0.27[0.22,0.33]} \\
gpt-4.1 vs gpt-4o-mini & 1.63[1.41,1.87] & 17.68[16.25,19.09] & 1.63[1.36,1.90] & 0.32[0.26,0.38] & 0.31[0.25,0.38] & \textbf{0.31[0.25,0.37]} \\
gpt-4.1 vs gpt-4o & 1.88[1.69,2.10] & 13.25[11.67,14.84] & 1.07[0.92,1.24] & 0.32[0.24,0.41] & \textbf{0.31[0.23,0.39]} & 0.31[0.23,0.39] \\
gpt-4.1-mini vs gpt-4o & 1.88[1.65,2.10] & 13.12[11.62,14.61] & 1.05[0.88,1.22] & 0.31[0.24,0.40] & 0.31[0.24,0.40] & \textbf{0.31[0.24,0.40]} \\
gpt-4.1 vs gpt-4.1-mini & 2.21[1.93,2.47] & 11.93[10.31,13.50] & 1.21[0.98,1.47] & 0.62[0.51,0.72] & 0.62[0.51,0.72] & \textbf{0.51[0.42,0.61]} \\
gpt-4o-mini vs gpt-4o-mini & 1.67[1.40,1.95] & 14.10[12.61,15.64] & 0.94[0.76,1.15] & 0.54[0.46,0.63] & 0.53[0.45,0.62] & \textbf{0.52[0.44,0.61]} \\
gpt-4o-mini vs gpt-5 & 2.66[2.49,2.85] & 8.36[7.03,9.61] & 1.27[1.07,1.47] & 0.61[0.56,0.67] & 0.59[0.54,0.65] & \textbf{0.53[0.49,0.59]} \\
gpt-4.1-mini vs gpt-4.1-mini & 2.30[2.02,2.59] & 10.59[9.06,12.14] & 1.05[0.86,1.27] & 0.61[0.51,0.72] & 0.61[0.51,0.72] & \textbf{0.53[0.45,0.64]} \\
gpt-4o-mini vs gpt-5-mini & 2.78[2.60,2.96] & 8.65[7.23,10.06] & 1.40[1.19,1.61] & 0.65[0.61,0.71] & 0.65[0.61,0.71] & \textbf{0.57[0.53,0.64]} \\
gpt-4.1 vs gpt-5-mini & 2.88[2.68,3.09] & 9.21[7.56,10.79] & 1.37[1.16,1.60] & 0.69[0.61,0.76] & 0.68[0.60,0.76] & \textbf{0.61[0.53,0.69]} \\
gpt-4.1 vs gpt-4.1 & 2.36[2.10,2.67] & 10.75[9.13,12.27] & 1.21[0.96,1.45] & 0.86[0.79,0.95] & 0.86[0.79,0.95] & \textbf{0.64[0.56,0.74]} \\
gpt-4o vs gpt-5-mini & 3.00[2.78,3.24] & 8.86[7.30,10.36] & 1.38[1.18,1.59] & 0.73[0.64,0.83] & 0.72[0.63,0.82] & \textbf{0.65[0.56,0.75]} \\
gpt-4.1-mini vs gpt-5-mini & 3.06[2.87,3.26] & 9.56[7.94,11.25] & 1.52[1.31,1.75] & 0.76[0.69,0.84] & 0.75[0.68,0.82] & \textbf{0.66[0.59,0.73]} \\
gpt-4.1 vs gpt-5 & 3.06[2.85,3.28] & 8.06[6.53,9.55] & 1.41[1.21,1.62] & 0.74[0.67,0.82] & 0.73[0.66,0.82] & \textbf{0.66[0.59,0.74]} \\
gpt-4.1-mini vs gpt-5 & 3.17[2.94,3.39] & 8.12[6.62,9.65] & 1.36[1.16,1.57] & 0.78[0.68,0.87] & 0.75[0.66,0.84] & \textbf{0.68[0.58,0.77]} \\
gpt-4o vs gpt-5 & 3.08[2.87,3.29] & 6.51[5.27,7.82] & 1.22[1.06,1.40] & 0.75[0.67,0.83] & 0.75[0.67,0.83] & \textbf{0.70[0.62,0.77]} \\
gpt-5 vs gpt-5-mini & 5.05[4.91,5.16] & \textbf{0.03[0.01,0.09]} & 1.49[1.40,1.55] & 1.49[1.40,1.55] & 1.49[1.40,1.55] & 1.44[1.36,1.50] \\
gpt-5-mini vs gpt-5-mini & 5.08[4.94,5.20] & \textbf{0.02[0.00,0.07]} & 1.50[1.42,1.58] & 1.50[1.42,1.58] & 1.50[1.42,1.58] & 1.46[1.37,1.53] \\
gpt-5 vs gpt-5 & 5.12[5.01,5.20] & \textbf{0.01[0.00,0.04]} & 1.53[1.45,1.58] & 1.53[1.45,1.58] & 1.53[1.45,1.58] & 1.48[1.41,1.53] \\
\end{longtable}}
