# Supplementary material for: Correlated Quantal Response Equilibrium: A New Equilibrium Notion for Human-AI Strategic Interactions
Source: arXiv:2610.29020 source file (2026-10-21)
Supplement: Supplementary file 9 [file sm_n5_ci.tex]

{\scriptsize\setlength{\tabcolsep}{2.5pt}\renewcommand{\arraystretch}{1.05}
\begin{longtable}{lrrrrrr}
\caption{Per-pair mean KL with 95\,\% bootstrap CI for game \texttt{sm\_n5}. Each cell is ``mean\,[lo,\,hi]'' in nats. Pairs sorted ascending by CQRE-pa mean. Boldface marks the lowest-mean equilibrium notion in each row.}\label{tab:appendix_ci_sm_n5}\\
\toprule
Model pair & Nash & Logit-QRE & Exact CQRE & CQRE sc. & CQRE pp. & CQRE-pa \\
\midrule
\endfirsthead
\multicolumn{7}{l}{\textit{(continued)}}\\
\toprule
Model pair & Nash & Logit-QRE & Exact CQRE & CQRE sc. & CQRE pp. & CQRE-pa \\
\midrule
\endhead
\bottomrule
\endfoot
gpt-4.1 vs gpt-4o & 9.93[8.48,11.52] & 0.24[0.17,0.33] & 2.04[1.71,2.40] & 0.23[0.16,0.31] & 0.23[0.16,0.31] & \textbf{0.20[0.14,0.28]} \\
gpt-4.1-mini vs gpt-4o & 6.35[5.09,7.69] & 0.38[0.29,0.48] & 2.47[2.13,2.81] & 0.38[0.29,0.48] & 0.37[0.28,0.47] & \textbf{0.30[0.22,0.39]} \\
gpt-4.1 vs gpt-4o-mini & 6.47[5.12,7.86] & 0.39[0.30,0.51] & 2.96[2.59,3.35] & 0.38[0.28,0.49] & 0.36[0.27,0.47] & \textbf{0.34[0.25,0.44]} \\
gpt-4o vs gpt-4o & 7.51[6.06,9.00] & 0.50[0.40,0.61] & 1.66[1.36,1.96] & 0.48[0.38,0.58] & 0.44[0.35,0.54] & \textbf{0.36[0.27,0.46]} \\
gpt-4.1 vs gpt-4.1-mini & 5.63[4.48,6.77] & 0.49[0.39,0.61] & 2.44[2.14,2.76] & 0.49[0.39,0.61] & 0.48[0.38,0.59] & \textbf{0.39[0.30,0.48]} \\
gpt-4o vs gpt-4o-mini & 5.58[4.40,6.79] & 0.53[0.42,0.67] & 2.30[1.99,2.64] & 0.52[0.41,0.65] & 0.51[0.40,0.64] & \textbf{0.47[0.36,0.59]} \\
gpt-4.1 vs gpt-4.1 & 5.56[4.42,6.89] & 0.66[0.54,0.79] & 1.77[1.51,2.06] & 0.62[0.51,0.75] & 0.60[0.49,0.71] & \textbf{0.53[0.42,0.64]} \\
gpt-4.1-mini vs gpt-4o-mini & 5.19[4.15,6.37] & 0.63[0.51,0.77] & 2.90[2.57,3.27] & 0.63[0.51,0.77] & 0.63[0.51,0.77] & \textbf{0.55[0.44,0.68]} \\
gpt-4.1 vs gpt-5-mini & 6.75[5.37,8.09] & 0.78[0.67,0.89] & 2.43[2.07,2.79] & 0.76[0.66,0.88] & 0.76[0.66,0.87] & \textbf{0.71[0.59,0.83]} \\
gpt-4.1-mini vs gpt-4.1-mini & 5.90[4.67,7.00] & 0.85[0.71,0.98] & 3.34[3.04,3.64] & 0.85[0.71,0.98] & 0.84[0.70,0.97] & \textbf{0.72[0.60,0.83]} \\
gpt-4o vs gpt-5-mini & 5.21[3.96,6.56] & 0.82[0.73,0.93] & 2.25[1.95,2.60] & 0.82[0.72,0.93] & 0.81[0.71,0.92] & \textbf{0.78[0.67,0.88]} \\
gpt-4o-mini vs gpt-4o-mini & 5.67[4.61,6.84] & 0.90[0.76,1.07] & 2.76[2.46,3.08] & 0.89[0.76,1.04] & 0.87[0.73,1.00] & \textbf{0.81[0.67,0.95]} \\
gpt-4.1-mini vs gpt-5-mini & 3.55[2.67,4.59] & 0.97[0.86,1.07] & 3.08[2.72,3.48] & 0.97[0.86,1.07] & 0.94[0.83,1.04] & \textbf{0.89[0.78,1.00]} \\
gpt-4o-mini vs gpt-5-mini & 4.83[3.77,5.91] & 1.02[0.90,1.14] & 3.59[3.18,4.01] & 0.97[0.86,1.09] & 0.95[0.84,1.07] & \textbf{0.91[0.80,1.02]} \\
gpt-4.1 vs gpt-5 & 5.04[3.71,6.25] & 1.12[1.04,1.22] & 2.52[2.22,2.85] & 1.09[1.01,1.17] & 1.08[1.00,1.17] & \textbf{1.03[0.95,1.11]} \\
gpt-4o vs gpt-5 & 4.94[3.78,6.28] & 1.08[0.99,1.18] & 2.52[2.19,2.88] & 1.07[0.98,1.17] & 1.06[0.97,1.16] & \textbf{1.03[0.94,1.13]} \\
gpt-4.1-mini vs gpt-5 & 3.67[2.84,4.60] & 1.39[1.29,1.49] & 3.87[3.44,4.27] & 1.38[1.28,1.48] & 1.33[1.24,1.42] & \textbf{1.30[1.21,1.40]} \\
gpt-4o-mini vs gpt-5 & 3.68[2.90,4.53] & 1.44[1.31,1.57] & 4.25[3.82,4.67] & 1.39[1.27,1.51] & 1.38[1.26,1.49] & \textbf{1.33[1.22,1.44]} \\
gpt-5-mini vs gpt-5-mini & 4.47[3.56,5.51] & 2.27[2.13,2.43] & 2.50[2.33,2.67] & 2.10[1.97,2.23] & 2.06[1.93,2.20] & \textbf{1.84[1.69,1.99]} \\
gpt-5 vs gpt-5-mini & 3.14[2.58,3.84] & 2.52[2.36,2.67] & 2.70[2.55,2.86] & 2.30[2.16,2.43] & 2.29[2.15,2.43] & \textbf{2.12[1.98,2.25]} \\
gpt-5 vs gpt-5 & 2.82[2.66,3.08] & 3.00[2.88,3.11] & 3.19[3.09,3.31] & 2.73[2.62,2.83] & 2.73[2.61,2.83] & \textbf{2.54[2.43,2.64]} \\
\end{longtable}}
