# Supplementary material for: Correlated Quantal Response Equilibrium: A New Equilibrium Notion for Human-AI Strategic Interactions
Source: arXiv:2610.29020 source file (2026-10-21)
Supplement: Supplementary file 10 [file sm_n7_ci.tex]

{\scriptsize\setlength{\tabcolsep}{2.5pt}\renewcommand{\arraystretch}{1.05}
\begin{longtable}{lrrrrrr}
\caption{Per-pair mean KL with 95\,\% bootstrap CI for game \texttt{sm\_n7}. Each cell is ``mean\,[lo,\,hi]'' in nats. Pairs sorted ascending by CQRE-pa mean. Boldface marks the lowest-mean equilibrium notion in each row.}\label{tab:appendix_ci_sm_n7}\\
\toprule
Model pair & Nash & Logit-QRE & Exact CQRE & CQRE sc. & CQRE pp. & CQRE-pa \\
\midrule
\endfirsthead
\multicolumn{7}{l}{\textit{(continued)}}\\
\toprule
Model pair & Nash & Logit-QRE & Exact CQRE & CQRE sc. & CQRE pp. & CQRE-pa \\
\midrule
\endhead
\bottomrule
\endfoot
gpt-4.1 vs gpt-4o & 7.59[6.17,9.02] & 0.53[0.43,0.65] & 1.28[1.07,1.51] & 0.53[0.43,0.65] & 0.53[0.43,0.65] & \textbf{0.48[0.38,0.58]} \\
gpt-4o vs gpt-4o & 6.49[5.32,7.85] & 0.56[0.44,0.68] & 1.34[1.13,1.55] & 0.56[0.44,0.68] & 0.55[0.44,0.68] & \textbf{0.52[0.41,0.65]} \\
gpt-4.1 vs gpt-4.1 & 8.65[7.24,10.15] & 0.67[0.56,0.78] & 1.25[1.06,1.47] & 0.67[0.56,0.78] & 0.64[0.54,0.75] & \textbf{0.55[0.45,0.65]} \\
gpt-4.1-mini vs gpt-4o & 5.17[4.08,6.32] & 0.64[0.53,0.77] & 1.62[1.40,1.84] & 0.64[0.53,0.77] & 0.64[0.53,0.77] & \textbf{0.59[0.49,0.71]} \\
gpt-4o vs gpt-4o-mini & 7.19[5.94,8.55] & 0.64[0.51,0.78] & 1.68[1.46,1.91] & 0.64[0.51,0.78] & 0.64[0.51,0.78] & \textbf{0.59[0.48,0.71]} \\
gpt-4.1 vs gpt-4o-mini & 7.13[5.79,8.47] & 0.69[0.58,0.82] & 1.61[1.41,1.84] & 0.69[0.58,0.82] & 0.69[0.58,0.82] & \textbf{0.63[0.53,0.74]} \\
gpt-4.1 vs gpt-4.1-mini & 6.66[5.25,8.02] & 0.80[0.68,0.94] & 1.46[1.25,1.67] & 0.80[0.68,0.94] & 0.79[0.66,0.92] & \textbf{0.68[0.57,0.80]} \\
gpt-4.1-mini vs gpt-4o-mini & 6.74[5.53,8.13] & 0.91[0.78,1.05] & 1.95[1.75,2.15] & 0.91[0.78,1.05] & 0.90[0.78,1.05] & \textbf{0.85[0.73,0.97]} \\
gpt-4.1-mini vs gpt-4.1-mini & 4.08[3.24,5.07] & 1.23[1.10,1.35] & 2.05[1.83,2.28] & 1.23[1.10,1.35] & 1.20[1.09,1.33] & \textbf{1.06[0.95,1.19]} \\
gpt-4o-mini vs gpt-4o-mini & 6.29[5.14,7.47] & 1.28[1.09,1.47] & 1.88[1.68,2.09] & 1.28[1.09,1.47] & 1.27[1.08,1.46] & \textbf{1.14[0.96,1.31]} \\
gpt-4o vs gpt-5-mini & 22.84[21.85,23.77] & 1.24[1.12,1.36] & 1.99[1.80,2.19] & 1.21[1.10,1.32] & 1.20[1.09,1.32] & \textbf{1.17[1.06,1.29]} \\
gpt-4.1 vs gpt-5-mini & 22.61[21.50,23.69] & 1.36[1.24,1.49] & 1.97[1.79,2.15] & 1.30[1.19,1.43] & 1.30[1.19,1.43] & \textbf{1.25[1.14,1.36]} \\
gpt-4.1-mini vs gpt-5-mini & 22.77[21.61,23.82] & 1.51[1.37,1.65] & 2.38[2.18,2.59] & 1.46[1.33,1.60] & 1.45[1.32,1.59] & \textbf{1.39[1.26,1.53]} \\
gpt-4o-mini vs gpt-5-mini & 22.90[21.80,23.88] & 1.51[1.37,1.64] & 2.47[2.23,2.69] & 1.48[1.34,1.61] & 1.47[1.33,1.61] & \textbf{1.41[1.27,1.54]} \\
gpt-4o vs gpt-5 & 25.31[25.23,25.42] & 1.58[1.49,1.68] & 2.23[2.07,2.40] & 1.51[1.42,1.60] & 1.51[1.42,1.60] & \textbf{1.48[1.39,1.57]} \\
gpt-4.1 vs gpt-5 & 25.44[25.35,25.55] & 1.70[1.61,1.81] & 2.26[2.11,2.42] & 1.64[1.54,1.73] & 1.63[1.55,1.73] & \textbf{1.57[1.49,1.67]} \\
gpt-4o-mini vs gpt-5 & 25.46[25.38,25.56] & 1.72[1.64,1.82] & 2.70[2.52,2.89] & 1.68[1.60,1.78] & 1.68[1.60,1.78] & \textbf{1.63[1.55,1.72]} \\
gpt-4.1-mini vs gpt-5 & 25.51[25.20,25.73] & 1.88[1.76,2.01] & 2.90[2.72,3.10] & 1.84[1.72,1.96] & 1.84[1.72,1.96] & \textbf{1.77[1.65,1.90]} \\
gpt-5-mini vs gpt-5-mini & 26.65[26.27,26.94] & 3.03[2.85,3.22] & 2.59[2.47,2.71] & 2.59[2.47,2.71] & 2.59[2.47,2.71] & \textbf{2.45[2.33,2.58]} \\
gpt-5 vs gpt-5-mini & 27.00[26.82,27.17] & 3.26[3.08,3.43] & 2.74[2.64,2.85] & 2.74[2.64,2.85] & 2.74[2.64,2.85] & \textbf{2.64[2.53,2.76]} \\
gpt-5 vs gpt-5 & 27.57[27.50,27.63] & 3.83[3.76,3.89] & 3.11[3.05,3.15] & 3.11[3.05,3.15] & 3.11[3.05,3.15] & \textbf{3.04[2.98,3.08]} \\
\end{longtable}}
